# Supplementary material for: Sharp nonparametric bounds for decomposition effects with two binary mediators
Source: arXiv:2112.13632 ancillary file (2021-12-27)
Supplement: Supplementary file 1 [file supplement.pdf]

# Sharp nonparametric bounds for decomposition effects with two mediators – Supplemental Materials

Erin E Gabriel Michael C Sachs Arvid Sjölander

2021-03-16

## Notation and estimands

Here we reproduce the decompositions of the total effect as reported in Daniel et al. 2015, Table 2. Each element of the decomposition is a link to the bounds for that element. The total effect is $\text{TE} = p\{Y(1) = 1\} - p\{Y(0) = 1\}$. The terms of the decomposition are defined as follows for $x, x_1, x_2, x_3 \in \{0, 1\}$:

The natural direct effect:

$$\begin{aligned}\text{NDE-}x_1x_2x_3 &= p\{Y(1, M_1(x_1), M_2(x_2, M_1(x_3))) = 1\} \\ &- p\{Y(0, M_1(x_1), M_2(x_2, M_1(x_3))) = 1\}.\end{aligned}$$

The indirect effect through $M_1$ only:

$$\begin{aligned}\text{NIE}_1\text{-}xx_2x_3 &= p\{Y(x, M_1(1), M_2(x_2, M_1(x_3))) = 1\} \\ &- p\{Y(x, M_1(0), M_2(x_2, M_1(x_3))) = 1\}.\end{aligned}$$

The indirect effect through $M_2$ only:

$$\begin{aligned}\text{NIE}_2\text{-}xx_1x_3 &= p\{Y(x, M_1(x_1), M_2(1, M_1(x_3))) = 1\} \\ &- p\{Y(x, M_1(x_1), M_2(0, M_1(x_3))) = 1\}.\end{aligned}$$

The indirect effect through both $M_1$ and $M_2$

$$\begin{aligned}\text{NIE}_{12}\text{-}xx_1x_2 &= p\{Y(x, M_1(x_1), M_2(x_2, M_1(1))) = 1\} \\ &- p\{Y(x, M_1(x_1), M_2(x_2, M_1(0))) = 1\}.\end{aligned}$$

Define the short hand notation for the estimable probabilities as:

$$p_{ym_1m_2\cdot x} = p\{Y = y, M_1 = m_1, M_2 = m_2 | X = x\}.$$

For example, $p_{111\cdot 1} = p\{Y = 1, M_1 = 1, M_2 = 1 | X = 1\}$.

## Decompositions

TE = NDE-000 + $\text{NIE}_1$-100 + $\text{NIE}_2$-110 + $\text{NIE}_{12}$-111

TE = NDE-000 + $\text{NIE}_1$-100 + $\text{NIE}_2$-111 + $\text{NIE}_{12}$-110

TE = NDE-000 + $\text{NIE}_1$-110 + $\text{NIE}_2$-100 + $\text{NIE}_{12}$-111

TE = NDE-000 + $\text{NIE}_1$-101 + $\text{NIE}_2$-111 + $\text{NIE}_{12}$-100

TE = NDE-000 + $\text{NIE}_1$-111 + $\text{NIE}_2$-100 + $\text{NIE}_{12}$-101

TE = NDE-000 + $\text{NIE}_1$-111 + $\text{NIE}_2$-101 + $\text{NIE}_{12}$-100

TE = NDE-100 + $\text{NIE}_1$-000 + $\text{NIE}_2$-110 + $\text{NIE}_{12}$-111

TE = NDE-100 + $\text{NIE}_1$-000 + $\text{NIE}_2$-111 + $\text{NIE}_{12}$-110

TE = NDE-010 + $\text{NIE}_1$-110 + $\text{NIE}_2$-000 + $\text{NIE}_{12}$-111

TE = NDE-010 + $\text{NIE}_1$-111 + $\text{NIE}_2$-000 + $\text{NIE}_{12}$-101

TE = NDE-001 + $\text{NIE}_1$-101 + $\text{NIE}_2$-111 + $\text{NIE}_{12}$-000

TE = NDE-001 + $\text{NIE}_1$-111 + $\text{NIE}_2$-101 + $\text{NIE}_{12}$-000

TE = NDE-110 + $\text{NIE}_1$-000 + $\text{NIE}_2$-010 + $\text{NIE}_{12}$-111

TE = NDE-110 + $\text{NIE}_1$-010 + $\text{NIE}_2$-000 + $\text{NIE}_{12}$-111

TE = NDE-101 + $\text{NIE}_1$-000 + $\text{NIE}_2$-111 + $\text{NIE}_{12}$-010

TE = NDE-101 + $\text{NIE}_1$-001 + $\text{NIE}_2$-111 + $\text{NIE}_{12}$-000

TE = NDE-011 + $\text{NIE}_1$-111 + $\text{NIE}_2$-000 + $\text{NIE}_{12}$-001

TE = NDE-011 + $\text{NIE}_1$-111 + $\text{NIE}_2$-001 + $\text{NIE}_{12}$-000

TE = NDE-111 + $\text{NIE}_1$-000 + $\text{NIE}_2$-010 + $\text{NIE}_{12}$-011

TE = NDE-111 + $\text{NIE}_1$-000 + $\text{NIE}_2$-011 + $\text{NIE}_{12}$-010

TE = NDE-111 + $\text{NIE}_1$-010 + $\text{NIE}_2$-000 + $\text{NIE}_{12}$-011

TE = NDE-111 + $\text{NIE}_1$-001 + $\text{NIE}_2$-011 + $\text{NIE}_{12}$-000

TE = NDE-111 + $\text{NIE}_1$-011 + $\text{NIE}_2$-000 + $\text{NIE}_{12}$-001

TE = NDE-111 + $\text{NIE}_1$-011 + $\text{NIE}_2$-001 + $\text{NIE}_{12}$-000

# Bounds and bounds functions

## NDE-000

Lower bound =

$$\max\left\{\begin{array}{l}-p_{000\cdot 1}-p_{100\cdot 0}-p_{100\cdot 1}-p_{010\cdot 1}-p_{110\cdot 0}-p_{110\cdot 1}-p_{001\cdot 1}-p_{101\cdot 0}-p_{101\cdot 1}+p_{011\cdot 0}-p_{011\cdot 1},\\ -2+p_{000\cdot 0}+p_{010\cdot 0}+2p_{001\cdot 0}+p_{101\cdot 0}+p_{101\cdot 1}+p_{011\cdot 0},\\ -2+p_{000\cdot 0}+2p_{010\cdot 0}+p_{110\cdot 0}+p_{110\cdot 1}+p_{001\cdot 0}+p_{011\cdot 0},\\ -2+2p_{000\cdot 0}+p_{100\cdot 0}+p_{100\cdot 1}+p_{010\cdot 0}+p_{001\cdot 0}+p_{011\cdot 0},\\ -1+p_{000\cdot 0}+p_{010\cdot 0}+p_{001\cdot 0}+p_{011\cdot 0}\end{array}\right\}$$

Upper bound =

$$\min\left\{\begin{array}{l}1+p_{000\cdot 0}-p_{010\cdot 1}-p_{110\cdot 0}+p_{001\cdot 0}+p_{011\cdot 0},\\ 1+p_{000\cdot 0}+p_{010\cdot 0}-p_{001\cdot 1}-p_{101\cdot 0}+p_{011\cdot 0},\\ 2p_{000\cdot 0}+p_{100\cdot 0}+2p_{010\cdot 0}+p_{110\cdot 0}+2p_{001\cdot 0}+p_{101\cdot 0}+p_{011\cdot 0}-p_{011\cdot 1},\\ p_{000\cdot 0}+p_{010\cdot 0}+p_{001\cdot 0}+p_{011\cdot 0},\\ 1-p_{000\cdot 1}-p_{100\cdot 0}+p_{010\cdot 0}+p_{001\cdot 0}+p_{011\cdot 0}\end{array}\right\}$$

Download R function for this bound (Double-click)

Back to top

## NIE$_1$-000

Lower bound =

$$\max\left\{\begin{array}{l}-p_{000\cdot 1}-p_{100\cdot 0}-p_{100\cdot 1}-p_{001\cdot 1}-p_{101\cdot 0}-p_{101\cdot 1},\\ -1+p_{000\cdot 0}+p_{010\cdot 0}+p_{001\cdot 0}+p_{011\cdot 0},\\ -2+p_{000\cdot 0}+p_{000\cdot 1}+p_{100\cdot 0}+p_{100\cdot 1}+p_{010\cdot 0}+p_{001\cdot 0}+p_{001\cdot 1}+p_{101\cdot 0}+p_{101\cdot 1}+p_{011\cdot 0}\end{array}\right\}$$

Upper bound =

$$\min\left\{\begin{array}{l}1-p_{000\cdot 1}-p_{100\cdot 1}+p_{010\cdot 0}-p_{001\cdot 1}-p_{101\cdot 1}+p_{011\cdot 0},\\ p_{000\cdot 0}+p_{010\cdot 0}+p_{001\cdot 0}+p_{011\cdot 0},\\ p_{000\cdot 0}+p_{000\cdot 1}+p_{100\cdot 1}+p_{001\cdot 0}+p_{001\cdot 1}+p_{101\cdot 1}\end{array}\right\}$$

Download R function for this bound (Double-click)

Back to top

## NIE$_2$-000

Lower bound =

$$\max\left\{\begin{array}{l}-p_{000\cdot1}-p_{100\cdot0}-p_{100\cdot1}-p_{010\cdot1}-p_{110\cdot0}-p_{110\cdot1}-p_{001\cdot1}-p_{101\cdot0}-p_{101\cdot1},\\ -1+p_{000\cdot0}+p_{010\cdot0}+p_{001\cdot0}+p_{011\cdot0},\\ -2+p_{000\cdot0}+p_{010\cdot0}+p_{001\cdot0}+p_{001\cdot1}+p_{101\cdot0}+p_{101\cdot1}+p_{011\cdot0},\\ -2+p_{000\cdot0}+p_{010\cdot0}+p_{010\cdot1}+p_{110\cdot0}+p_{110\cdot1}+p_{001\cdot0}+p_{011\cdot0},\\ -2+p_{000\cdot0}+p_{000\cdot1}+p_{100\cdot0}+p_{100\cdot1}+p_{010\cdot0}+p_{001\cdot0}+p_{011\cdot0}\end{array}\right\}$$

Upper bound =

$$\min\left\{\begin{array}{l}1-p_{000\cdot1}-p_{100\cdot1}+p_{010\cdot0}+p_{001\cdot0}+p_{011\cdot0},\\ p_{000\cdot0}+p_{010\cdot0}+p_{001\cdot0}+p_{011\cdot0},\\ 1+p_{000\cdot0}-p_{010\cdot1}-p_{110\cdot1}+p_{001\cdot0}+p_{011\cdot0},\\ 1+p_{000\cdot0}+p_{010\cdot0}-p_{001\cdot1}-p_{101\cdot1}+p_{011\cdot0},\\ p_{000\cdot0}+p_{000\cdot1}+p_{100\cdot1}+p_{010\cdot0}+p_{010\cdot1}+p_{110\cdot1}+p_{001\cdot0}+p_{001\cdot1}+p_{101\cdot1}\end{array}\right\}$$

Download R function for this bound (Double-click)

Back to top

## NIE$_{12}$-000

Lower bound =

$$\max\left\{\begin{array}{l}-p_{000\cdot1}-p_{100\cdot0}-p_{100\cdot1}-p_{001\cdot1}-p_{101\cdot0}-p_{101\cdot1},\\ -1+p_{000\cdot0}+p_{010\cdot0}+p_{001\cdot0}+p_{011\cdot0},\\ -2+p_{000\cdot0}+p_{000\cdot1}+p_{100\cdot0}+p_{100\cdot1}+p_{010\cdot0}+p_{001\cdot0}+p_{001\cdot1}+p_{101\cdot0}+p_{101\cdot1}+p_{011\cdot0}\end{array}\right\}$$

Upper bound =

$$\min\left\{\begin{array}{l}1-p_{000\cdot1}-p_{100\cdot1}+p_{010\cdot0}-p_{001\cdot1}-p_{101\cdot1}+p_{011\cdot0},\\ p_{000\cdot0}+p_{010\cdot0}+p_{001\cdot0}+p_{011\cdot0},\\ p_{000\cdot0}+p_{000\cdot1}+p_{100\cdot1}+p_{001\cdot0}+p_{001\cdot1}+p_{101\cdot1}\end{array}\right\}$$

Download R function for this bound (Double-click)

Back to top

**NDE-100**

Lower bound =

$$\max\left\{\begin{array}{l}
-p_{000\cdot 0}-2p_{000\cdot 1}-p_{100\cdot 0}-2p_{100\cdot 1}-p_{010\cdot 1}-p_{110\cdot 0}-p_{110\cdot 1}-2p_{001\cdot 1}-p_{101\cdot 1}+p_{011\cdot 0}-p_{011\cdot 1},\\
-1-p_{100\cdot 0}-p_{010\cdot 0}-p_{010\cdot 1}-p_{110\cdot 0}-p_{110\cdot 1}+p_{001\cdot 0}+p_{101\cdot 1}-p_{011\cdot 1},\\
-2+p_{000\cdot 0}-p_{000\cdot 1}+p_{100\cdot 0}+2p_{010\cdot 0}+p_{110\cdot 0}+p_{110\cdot 1}-p_{001\cdot 1}-p_{101\cdot 1}+p_{011\cdot 0},\\
-3+2p_{000\cdot 0}+p_{000\cdot 1}+p_{100\cdot 0}+2p_{100\cdot 1}+p_{010\cdot 0}+p_{110\cdot 0}+p_{110\cdot 1}+p_{001\cdot 0}+p_{001\cdot 1}+p_{101\cdot 1},\\
-p_{000\cdot 0}-p_{000\cdot 1}-p_{100\cdot 0}-p_{100\cdot 1}-p_{010\cdot 0}-p_{010\cdot 1}-p_{110\cdot 0}-p_{110\cdot 1}-p_{001\cdot 1}-p_{011\cdot 1},\\
-p_{000\cdot 0}-p_{000\cdot 1}-p_{100\cdot 0}-p_{100\cdot 1}-p_{010\cdot 1}-p_{110\cdot 0}-p_{110\cdot 1}-p_{001\cdot 1}-p_{101\cdot 1}-p_{011\cdot 1},\\
-1-p_{000\cdot 1}-p_{100\cdot 1}-p_{001\cdot 1}+p_{011\cdot 0},\\
-1-p_{000\cdot 1}-p_{100\cdot 1}+p_{010\cdot 0}-p_{001\cdot 1}-p_{101\cdot 1}+p_{011\cdot 0},\\
-1-p_{100\cdot 0}-p_{010\cdot 0}-p_{110\cdot 0}+p_{101\cdot 1},\\
-2+p_{000\cdot 0}+p_{110\cdot 1}+p_{101\cdot 1}+p_{011\cdot 0},\\
-1-p_{010\cdot 1}-p_{110\cdot 1}+p_{001\cdot 0}-p_{011\cdot 1},\\
-1-p_{000\cdot 1}+p_{010\cdot 0}-p_{010\cdot 1}-p_{110\cdot 1}+p_{001\cdot 0}-p_{001\cdot 1}-p_{101\cdot 1}-p_{011\cdot 1},\\
-2+p_{000\cdot 0}+p_{000\cdot 1}+p_{100\cdot 1}+p_{001\cdot 0}+p_{001\cdot 1}+p_{101\cdot 1},\\
-2+p_{000\cdot 0}+p_{100\cdot 0}+p_{010\cdot 0}+p_{110\cdot 0}+p_{110\cdot 1}+p_{011\cdot 0},\\
-2+p_{000\cdot 0}+p_{100\cdot 0}+p_{100\cdot 1}+p_{010\cdot 0}+p_{110\cdot 0}+p_{110\cdot 1},\\
-1-p_{000\cdot 1}+p_{010\cdot 0}-p_{001\cdot 1}-p_{101\cdot 1},\\
-2+p_{000\cdot 0}+p_{100\cdot 0}+p_{100\cdot 1}+p_{010\cdot 0}+p_{110\cdot 0}+p_{001\cdot 0},\\
-2+p_{000\cdot 0}+p_{000\cdot 1}+p_{100\cdot 1}+p_{110\cdot 1}+p_{001\cdot 1}+p_{101\cdot 1},\\
-1
\end{array}\right\}$$

Upper bound =

$$\min\left\{\begin{array}{l}1 + p_{100\cdot1} - p_{010\cdot1} - p_{110\cdot0} + p_{001\cdot0} + p_{001\cdot1} + p_{101\cdot0} + p_{101\cdot1} + p_{011\cdot0},\\ 2 + p_{000\cdot0} - p_{000\cdot1} - p_{100\cdot1} + p_{010\cdot0} + p_{110\cdot0} - 2p_{001\cdot1} - p_{101\cdot0} - p_{101\cdot1} - p_{011\cdot1},\\ 2p_{000\cdot0} + p_{000\cdot1} + 2p_{100\cdot0} + p_{100\cdot1} + 2p_{010\cdot0} + p_{110\cdot0} + p_{001\cdot0} + p_{101\cdot0} + p_{101\cdot1} + p_{011\cdot0} - p_{011\cdot1},\\ 1,\\ 1 + p_{000\cdot0} + p_{100\cdot0} + p_{010\cdot0} + p_{110\cdot0} - p_{001\cdot1} - p_{011\cdot1},\\ 1 + p_{000\cdot0} + p_{100\cdot0} + p_{010\cdot0} - p_{011\cdot1},\\ p_{000\cdot0} + p_{000\cdot1} + p_{100\cdot0} + p_{100\cdot1} + p_{010\cdot0} + p_{110\cdot0} + p_{001\cdot0} + p_{101\cdot0} + p_{101\cdot1} + p_{011\cdot0},\\ p_{000\cdot0} + p_{000\cdot1} + p_{100\cdot0} + p_{100\cdot1} + p_{010\cdot0} + p_{001\cdot0} + p_{001\cdot1} + p_{101\cdot0} + p_{101\cdot1} + p_{011\cdot0},\\ 1 + p_{000\cdot0} + p_{010\cdot0} + p_{110\cdot0} - p_{001\cdot1},\\ 1 + p_{000\cdot0} + p_{010\cdot0} - p_{010\cdot1} + p_{110\cdot0} + p_{001\cdot0} - p_{001\cdot1} + p_{101\cdot0} + p_{011\cdot0},\\ 2 - p_{000\cdot1} - p_{100\cdot0} - p_{100\cdot1} - p_{010\cdot1} - p_{001\cdot1} - p_{101\cdot1},\\ 2 - p_{000\cdot1} - p_{100\cdot1} - p_{001\cdot1} - p_{101\cdot0} - p_{101\cdot1} - p_{011\cdot1},\\ 2 - p_{000\cdot1} - p_{100\cdot0} - p_{100\cdot1} - p_{001\cdot1} - p_{101\cdot0} - p_{101\cdot1},\\ 1 + p_{100\cdot1} - p_{110\cdot0} + p_{001\cdot1} + p_{101\cdot1},\\ 2 - p_{000\cdot1} - p_{110\cdot0} - p_{101\cdot0} - p_{011\cdot1},\\ 1 - p_{010\cdot1} + p_{001\cdot0} + p_{101\cdot0} + p_{011\cdot0},\\ 2 - p_{000\cdot0} - p_{000\cdot1} - p_{100\cdot0} - p_{010\cdot0} - p_{110\cdot0} - p_{101\cdot0},\\ 2 - p_{000\cdot0} - p_{000\cdot1} - p_{100\cdot0} - p_{010\cdot0} - p_{010\cdot1} - p_{110\cdot0},\\ 3 - p_{000\cdot0} - 2p_{000\cdot1} - 2p_{100\cdot0} - p_{100\cdot1} - p_{010\cdot0} - p_{010\cdot1} - p_{110\cdot0} - p_{001\cdot1} - p_{101\cdot0} - p_{101\cdot1}\end{array}\right\}$$

Download R function for this bound (Double-click)

Back to top

## $\text{NIE}_1$-100

Lower bound =

$$\max\left\{\begin{array}{l}
-p_{000\cdot 0} - p_{000\cdot 1} - p_{100\cdot 0} - p_{100\cdot 1} - p_{010\cdot 0} - p_{110\cdot 0} - p_{001\cdot 0} - p_{001\cdot 1} - p_{101\cdot 0},\\
-p_{000\cdot 0} - p_{000\cdot 1} - p_{100\cdot 0} - p_{100\cdot 1} - p_{001\cdot 0} - p_{001\cdot 1} - p_{101\cdot 0} - p_{101\cdot 1},\\
-p_{000\cdot 0} - p_{000\cdot 1} - p_{100\cdot 0} - p_{100\cdot 1} - p_{010\cdot 0} - p_{010\cdot 1} - p_{110\cdot 0} - p_{110\cdot 1} - p_{001\cdot 1} - p_{011\cdot 1},\\
-p_{000\cdot 0} - p_{000\cdot 1} - p_{100\cdot 0} - p_{100\cdot 1} - p_{010\cdot 1} - p_{110\cdot 1} - p_{001\cdot 1} - p_{101\cdot 1} - p_{011\cdot 1},\\
-1 - p_{010\cdot 0} - p_{110\cdot 0} + p_{110\cdot 1} - p_{001\cdot 0} - p_{101\cdot 0} + p_{101\cdot 1},\\
-1 - p_{010\cdot 0} - p_{110\cdot 0} + p_{101\cdot 1},\\
-1 - p_{010\cdot 1} - p_{110\cdot 1} + p_{001\cdot 0} + p_{101\cdot 0} - p_{011\cdot 1},\\
-1 - p_{000\cdot 1} + p_{010\cdot 0} - p_{010\cdot 1} + p_{110\cdot 0} - p_{110\cdot 1} + p_{001\cdot 0} - p_{001\cdot 1} + p_{101\cdot 0} - p_{101\cdot 1} - p_{011\cdot 1},\\
-2 + p_{000\cdot 0} + p_{000\cdot 1} + p_{100\cdot 0} + p_{100\cdot 1} + p_{001\cdot 0} + p_{001\cdot 1} + p_{101\cdot 0} + p_{101\cdot 1},\\
-1 + p_{110\cdot 1} - p_{001\cdot 0} - p_{101\cdot 0},\\
-1 - p_{000\cdot 1} + p_{010\cdot 0} + p_{110\cdot 0} - p_{001\cdot 1} - p_{101\cdot 1},\\
-2 + p_{000\cdot 0} + p_{100\cdot 0} + p_{100\cdot 1} + p_{010\cdot 0} + p_{110\cdot 0} + p_{110\cdot 1},\\
-2 + p_{000\cdot 0} + p_{100\cdot 0} + p_{100\cdot 1} + p_{010\cdot 0} + p_{110\cdot 0} + p_{001\cdot 0} + p_{101\cdot 0},\\
-2 + p_{000\cdot 0} + p_{000\cdot 1} + p_{100\cdot 0} + p_{100\cdot 1} + p_{110\cdot 1} + p_{001\cdot 1} + p_{101\cdot 1}
\end{array}\right\}$$

Upper bound =

$$\min\left\{\begin{array}{l}
2 - p_{000\cdot 0} - p_{000\cdot 1} - p_{100\cdot 0} - p_{100\cdot 1} - p_{010\cdot 1} - p_{001\cdot 1} - p_{101\cdot 1},\\
2 - p_{000\cdot 0} - p_{000\cdot 1} - p_{100\cdot 0} - p_{100\cdot 1} - p_{001\cdot 0} - p_{001\cdot 1} - p_{101\cdot 0} - p_{101\cdot 1},\\
2 - p_{000\cdot 0} - p_{000\cdot 1} - p_{100\cdot 0} - p_{010\cdot 0} - p_{010\cdot 1} - p_{110\cdot 0},\\
2 - p_{000\cdot 0} - p_{000\cdot 1} - p_{100\cdot 0} - p_{010\cdot 0} - p_{110\cdot 0} - p_{001\cdot 0} - p_{101\cdot 0},\\
1 + p_{010\cdot 0} - p_{010\cdot 1} + p_{110\cdot 0} + p_{001\cdot 0} - p_{001\cdot 1} + p_{101\cdot 0},\\
1 - p_{010\cdot 1} + p_{001\cdot 0} + p_{101\cdot 0},\\
1 + p_{010\cdot 0} + p_{110\cdot 0} - p_{001\cdot 1},\\
2 - p_{000\cdot 1} - p_{010\cdot 0} - p_{110\cdot 0} - p_{001\cdot 0} - p_{101\cdot 0} - p_{011\cdot 1},\\
1 + p_{100\cdot 1} - p_{010\cdot 0} - p_{110\cdot 0} + p_{001\cdot 1} + p_{101\cdot 1},\\
2 - p_{000\cdot 1} - p_{100\cdot 1} - p_{001\cdot 0} - p_{001\cdot 1} - p_{101\cdot 0} - p_{101\cdot 1} - p_{011\cdot 1},\\
p_{000\cdot 0} + p_{000\cdot 1} + p_{100\cdot 0} + p_{100\cdot 1} + p_{001\cdot 0} + p_{001\cdot 1} + p_{101\cdot 0} + p_{101\cdot 1},\\
1 + p_{000\cdot 0} + p_{100\cdot 0} - p_{011\cdot 1},\\
p_{000\cdot 0} + p_{000\cdot 1} + p_{100\cdot 0} + p_{100\cdot 1} + p_{010\cdot 0} + p_{110\cdot 0} + p_{001\cdot 0} + p_{101\cdot 0} + p_{101\cdot 1},\\
1 + p_{000\cdot 0} + p_{100\cdot 0} + p_{010\cdot 0} + p_{110\cdot 0} - p_{001\cdot 1} - p_{011\cdot 1}
\end{array}\right\}$$

Download R function for this bound (Double-click)

Back to top

## $\mathbf{NIE_2}$-100

Lower bound =

$$\max\left\{\begin{array}{l}-p_{000\cdot0}-p_{000\cdot1}-p_{100\cdot0}-p_{100\cdot1}-p_{010\cdot0}-p_{010\cdot1}-p_{110\cdot0}-p_{001\cdot0}-p_{001\cdot1}-p_{101\cdot0}-p_{101\cdot1},\\ -p_{000\cdot0}-p_{000\cdot1}-p_{100\cdot0}-p_{100\cdot1}-p_{010\cdot1}-p_{001\cdot0}-p_{001\cdot1}-p_{101\cdot0}-p_{101\cdot1}-p_{011\cdot1},\\ -2+p_{100\cdot1}+p_{001\cdot0}+p_{001\cdot1}+p_{101\cdot0}+p_{101\cdot1},\\ -2+p_{000\cdot0}+p_{100\cdot0}+p_{100\cdot1}+p_{001\cdot0}+p_{101\cdot0}+p_{101\cdot1},\\ -1-p_{000\cdot1}-p_{100\cdot1}+p_{010\cdot0}+p_{110\cdot0}-p_{001\cdot1}-p_{101\cdot1}-p_{011\cdot1},\\ -2+p_{000\cdot0}+p_{000\cdot1}+p_{100\cdot0}+p_{100\cdot1}+p_{101\cdot1},\\ -1\end{array}\right\}$$

Upper bound =

$$\min\left\{\begin{array}{l}2-p_{000\cdot0}-p_{000\cdot1}-p_{100\cdot0}-p_{100\cdot1}-p_{001\cdot1},\\ 2-p_{000\cdot0}-p_{000\cdot1}-p_{100\cdot0}-p_{001\cdot0}-p_{001\cdot1}-p_{101\cdot0},\\ 2-p_{000\cdot1}-p_{001\cdot0}-p_{001\cdot1}-p_{101\cdot0}-p_{101\cdot1},\\ 2-p_{010\cdot0}-p_{010\cdot1}-p_{110\cdot0}-p_{110\cdot1}-p_{011\cdot1},\\ 1+p_{000\cdot0}+p_{100\cdot0}-p_{010\cdot1}+p_{001\cdot0}+p_{101\cdot0}-p_{011\cdot1},\\ p_{000\cdot0}+p_{000\cdot1}+p_{100\cdot0}+p_{100\cdot1}+p_{010\cdot0}+p_{110\cdot0}+p_{110\cdot1}+p_{001\cdot0}+p_{001\cdot1}+p_{101\cdot0}+p_{101\cdot1},\\ 1\end{array}\right\}$$

Download R function for this bound (Double-click)

Back to top

## $\mathbf{NIE_{12}}$-100

Lower bound =

$$\max\left\{\begin{array}{l}-p_{000\cdot0}-p_{000\cdot1}-p_{100\cdot0}-p_{100\cdot1}-p_{001\cdot0}-p_{001\cdot1}-p_{101\cdot0}-p_{101\cdot1},\\ -2+p_{000\cdot0}+p_{000\cdot1}+p_{100\cdot0}+p_{100\cdot1}+p_{001\cdot0}+p_{001\cdot1}+p_{101\cdot0}+p_{101\cdot1}\end{array}\right\}$$

Upper bound =

$$\min\left\{\begin{array}{l}2-p_{000\cdot0}-p_{000\cdot1}-p_{100\cdot0}-p_{100\cdot1}-p_{001\cdot0}-p_{001\cdot1}-p_{101\cdot0}-p_{101\cdot1},\\ p_{000\cdot0}+p_{000\cdot1}+p_{100\cdot0}+p_{100\cdot1}+p_{001\cdot0}+p_{001\cdot1}+p_{101\cdot0}+p_{101\cdot1}\end{array}\right\}$$

Download R function for this bound (Double-click)

Back to top

## NDE-010

Lower bound =

$$\max \begin{Bmatrix} -p_{000\cdot0} - 2p_{000\cdot1} - p_{100\cdot0} - 2p_{100\cdot1} - 2p_{010\cdot1} - p_{110\cdot1} - p_{001\cdot0} - 2p_{001\cdot1} - p_{101\cdot0} - 2p_{101\cdot1} + p_{011\cdot0} - p_{011\cdot1}, \\ -3 + p_{000\cdot0} + p_{100\cdot0} + p_{100\cdot1} + 2p_{001\cdot0} + p_{001\cdot1} + p_{101\cdot0} + 2p_{101\cdot1}, \\ -1 - p_{000\cdot0} - p_{000\cdot1} - p_{100\cdot0} - p_{100\cdot1} + p_{010\cdot0} + p_{110\cdot1} - p_{001\cdot0} - p_{001\cdot1} - p_{101\cdot0} - p_{101\cdot1} - p_{011\cdot1}, \\ -3 + 2p_{000\cdot0} + p_{000\cdot1} + p_{100\cdot0} + 2p_{100\cdot1} + p_{001\cdot0} + p_{101\cdot0} + p_{101\cdot1}, \\ -p_{000\cdot0} - p_{000\cdot1} - p_{100\cdot0} - p_{100\cdot1} - p_{010\cdot1} - p_{001\cdot0} - p_{001\cdot1} - p_{101\cdot0} - p_{101\cdot1} - p_{011\cdot1}, \\ -1 - p_{000\cdot1} - p_{100\cdot1} - p_{010\cdot1} - p_{001\cdot1} - p_{101\cdot1} + p_{011\cdot0}, \\ -2 + p_{000\cdot0} + p_{100\cdot0} + p_{100\cdot1} + p_{001\cdot0} + p_{101\cdot0} + p_{101\cdot1}, \\ -2 + p_{100\cdot1} + p_{001\cdot0} + p_{001\cdot1} + p_{101\cdot1}, \\ -1 - p_{000\cdot1} - p_{100\cdot1} + p_{010\cdot0} - p_{001\cdot1} - p_{101\cdot1} - p_{011\cdot1}, \\ -2 + p_{000\cdot0} + p_{000\cdot1} + p_{100\cdot1} + p_{101\cdot1}, \\ -1 \end{Bmatrix}$$

Upper bound =

$$\min \begin{Bmatrix} 2 + p_{000\cdot0} + p_{100\cdot0} - 2p_{010\cdot1} - p_{110\cdot0} - p_{110\cdot1} + p_{001\cdot0} + p_{101\cdot0} - p_{011\cdot1}, \\ 3 - p_{000\cdot0} - p_{000\cdot1} - p_{100\cdot0} - p_{001\cdot0} - 2p_{001\cdot1} - 2p_{101\cdot0} - p_{101\cdot1}, \\ 2p_{000\cdot0} + p_{000\cdot1} + 2p_{100\cdot0} + p_{100\cdot1} + p_{010\cdot0} + p_{110\cdot0} + p_{110\cdot1} + 2p_{001\cdot0} + p_{001\cdot1} + 2p_{101\cdot0} + p_{101\cdot1} + p_{011\cdot0} - p_{011\cdot1}, \\ 1, \\ 2 - p_{010\cdot1} - p_{110\cdot0} - p_{110\cdot1} - p_{011\cdot1}, \\ p_{000\cdot0} + p_{000\cdot1} + p_{100\cdot0} + p_{100\cdot1} + p_{010\cdot0} + p_{110\cdot0} + p_{110\cdot1} + p_{001\cdot0} + p_{001\cdot1} + p_{101\cdot0} + p_{101\cdot1} + p_{011\cdot0}, \\ 1 + p_{000\cdot0} + p_{100\cdot0} - p_{010\cdot1} + p_{001\cdot0} + p_{101\cdot0} - p_{011\cdot1}, \\ 2 - p_{000\cdot1} - p_{100\cdot0} - p_{100\cdot1} - p_{001\cdot1}, \\ 2 - p_{000\cdot1} - p_{001\cdot1} - p_{101\cdot0} - p_{101\cdot1}, \\ 2 - p_{000\cdot0} - p_{000\cdot1} - p_{100\cdot0} - p_{001\cdot0} - p_{001\cdot1} - p_{101\cdot0}, \\ 3 - p_{000\cdot0} - 2p_{000\cdot1} - 2p_{100\cdot0} - p_{100\cdot1} - p_{001\cdot0} - p_{001\cdot1} - p_{101\cdot0} \end{Bmatrix}$$

Download R function for this bound (Double-click)

Back to top

## NIE$_1$-010

Lower bound =

$$\max \begin{Bmatrix} -p_{000\cdot0} - p_{000\cdot1} - p_{100\cdot0} - p_{100\cdot1} - p_{001\cdot0} - p_{001\cdot1} - p_{101\cdot0} - p_{101\cdot1}, \\ -2 + p_{000\cdot0} + p_{000\cdot1} + p_{100\cdot0} + p_{100\cdot1} + p_{001\cdot0} + p_{001\cdot1} + p_{101\cdot0} + p_{101\cdot1} \end{Bmatrix}$$

Upper bound =

$$\min \begin{Bmatrix} 2 - p_{000\cdot0} - p_{000\cdot1} - p_{100\cdot0} - p_{100\cdot1} - p_{001\cdot0} - p_{001\cdot1} - p_{101\cdot0} - p_{101\cdot1}, \\ p_{000\cdot0} + p_{000\cdot1} + p_{100\cdot0} + p_{100\cdot1} + p_{001\cdot0} + p_{001\cdot1} + p_{101\cdot0} + p_{101\cdot1} \end{Bmatrix}$$

Download R function for this bound (Double-click)

Back to top

## $\text{NIE}_2$-010

Lower bound =

$$\max \begin{Bmatrix} -p_{000\cdot0} - p_{000\cdot1} - p_{100\cdot0} - p_{100\cdot1} - p_{010\cdot1} - p_{110\cdot0} - p_{110\cdot1} - p_{001\cdot0} - p_{001\cdot1} - p_{101\cdot0} - p_{101\cdot1}, \\ -1 - p_{000\cdot1} - p_{100\cdot1} + p_{010\cdot0} - p_{001\cdot1} - p_{101\cdot1} + p_{011\cdot0}, \\ -2 + p_{000\cdot0} + p_{001\cdot0} + p_{001\cdot1} + p_{101\cdot0} + p_{101\cdot1}, \\ -2 + p_{000\cdot0} + p_{000\cdot1} + p_{100\cdot1} + p_{001\cdot0} + p_{001\cdot1} + p_{101\cdot1}, \\ -2 + p_{010\cdot0} + p_{010\cdot1} + p_{110\cdot0} + p_{110\cdot1} + p_{011\cdot0}, \\ -2 + p_{000\cdot0} + p_{000\cdot1} + p_{100\cdot0} + p_{100\cdot1} + p_{001\cdot0}, \\ -1 \end{Bmatrix}$$

Upper bound =

$$\min \begin{Bmatrix} 2 - p_{000\cdot0} - p_{000\cdot1} - p_{100\cdot0} - p_{100\cdot1} - p_{101\cdot0}, \\ 2 - p_{000\cdot1} - p_{100\cdot0} - p_{100\cdot1} - p_{001\cdot1} - p_{101\cdot0} - p_{101\cdot1}, \\ 2 - p_{100\cdot0} - p_{001\cdot0} - p_{001\cdot1} - p_{101\cdot0} - p_{101\cdot1}, \\ 1 + p_{000\cdot0} + p_{100\cdot0} - p_{010\cdot1} - p_{110\cdot1} + p_{001\cdot0} + p_{101\cdot0} + p_{011\cdot0}, \\ p_{000\cdot0} + p_{000\cdot1} + p_{100\cdot0} + p_{100\cdot1} + p_{010\cdot0} + p_{001\cdot0} + p_{001\cdot1} + p_{101\cdot0} + p_{101\cdot1} + p_{011\cdot0}, \\ p_{000\cdot0} + p_{000\cdot1} + p_{100\cdot0} + p_{100\cdot1} + p_{010\cdot0} + p_{010\cdot1} + p_{110\cdot1} + p_{001\cdot0} + p_{001\cdot1} + p_{101\cdot0} + p_{101\cdot1}, \\ 1 \end{Bmatrix}$$

Download R function for this bound (Double-click)

Back to top

## $\text{NIE}_{12}$-010

Lower bound =

$$\max \begin{Bmatrix} -p_{000\cdot0} - p_{000\cdot1} - p_{100\cdot0} - p_{100\cdot1} - p_{001\cdot0} - p_{001\cdot1} - p_{101\cdot0} - p_{101\cdot1}, \\ -2 + p_{000\cdot0} + p_{000\cdot1} + p_{100\cdot0} + p_{100\cdot1} + p_{001\cdot0} + p_{001\cdot1} + p_{101\cdot0} + p_{101\cdot1} \end{Bmatrix}$$

Upper bound =

$$\min \begin{Bmatrix} 2 - p_{000\cdot0} - p_{000\cdot1} - p_{100\cdot0} - p_{100\cdot1} - p_{001\cdot0} - p_{001\cdot1} - p_{101\cdot0} - p_{101\cdot1}, \\ p_{000\cdot0} + p_{000\cdot1} + p_{100\cdot0} + p_{100\cdot1} + p_{001\cdot0} + p_{001\cdot1} + p_{101\cdot0} + p_{101\cdot1} \end{Bmatrix}$$

Download R function for this bound (Double-click)

Back to top

## NDE-001

Lower bound =

$$\max\left\{\begin{array}{l}-p_{000\cdot 0}-2p_{000\cdot 1}-p_{100\cdot 0}-2p_{100\cdot 1}-p_{010\cdot 1}-p_{110\cdot 0}-p_{110\cdot 1}-p_{001\cdot 0}-2p_{001\cdot 1}-p_{101\cdot 0}-2p_{101\cdot 1}+p_{011\cdot 0}-p_{011\cdot 1},\\ -3+p_{000\cdot 0}+p_{000\cdot 1}+p_{100\cdot 1}+2p_{001\cdot 0}+p_{001\cdot 1}+p_{101\cdot 0}+2p_{101\cdot 1},\\ -2-p_{000\cdot 1}-p_{100\cdot 1}+2p_{010\cdot 0}+p_{110\cdot 0}+p_{110\cdot 1}-p_{001\cdot 1}-p_{101\cdot 1}+p_{011\cdot 0},\\ -3+2p_{000\cdot 0}+p_{000\cdot 1}+p_{100\cdot 0}+2p_{100\cdot 1}+p_{001\cdot 0}+p_{001\cdot 1}+p_{101\cdot 1},\\ -p_{000\cdot 0}-p_{000\cdot 1}-p_{100\cdot 0}-p_{100\cdot 1}-p_{010\cdot 1}-p_{110\cdot 0}-p_{110\cdot 1}-p_{001\cdot 0}-p_{001\cdot 1}-p_{101\cdot 0}-p_{101\cdot 1}-p_{011\cdot 1},\\ -1-p_{000\cdot 1}-p_{100\cdot 1}+p_{010\cdot 0}-p_{001\cdot 1}-p_{101\cdot 1}+p_{011\cdot 0},\\ -2+p_{000\cdot 0}+p_{001\cdot 0}+p_{101\cdot 0}+p_{101\cdot 1},\\ -2+p_{000\cdot 0}+p_{000\cdot 1}+p_{100\cdot 1}+p_{001\cdot 0}+p_{001\cdot 1}+p_{101\cdot 1},\\ -2+p_{010\cdot 0}+p_{110\cdot 0}+p_{110\cdot 1}+p_{011\cdot 0},\\ -2+p_{000\cdot 0}+p_{100\cdot 0}+p_{100\cdot 1}+p_{001\cdot 0},\\ -1\end{array}\right\}$$

Upper bound =

$$\min\left\{\begin{array}{l}1+p_{000\cdot 0}+p_{000\cdot 1}+p_{100\cdot 0}+p_{100\cdot 1}-p_{010\cdot 1}-p_{110\cdot 0}+p_{001\cdot 0}+p_{001\cdot 1}+p_{101\cdot 0}+p_{101\cdot 1}+p_{011\cdot 0},\\ 3-p_{000\cdot 1}-p_{100\cdot 0}-p_{100\cdot 1}-p_{001\cdot 0}-2p_{001\cdot 1}-2p_{101\cdot 0}-p_{101\cdot 1},\\ 2p_{000\cdot 0}+p_{000\cdot 1}+2p_{100\cdot 0}+p_{100\cdot 1}+2p_{010\cdot 0}+p_{110\cdot 0}+2p_{001\cdot 0}+p_{001\cdot 1}+2p_{101\cdot 0}+p_{101\cdot 1}+p_{011\cdot 0}-p_{011\cdot 1},\\ 1,\\ 1+p_{000\cdot 0}+p_{100\cdot 0}+p_{010\cdot 0}+p_{001\cdot 0}+p_{101\cdot 0}-p_{011\cdot 1},\\ p_{000\cdot 0}+p_{000\cdot 1}+p_{100\cdot 0}+p_{100\cdot 1}+p_{010\cdot 0}+p_{001\cdot 0}+p_{001\cdot 1}+p_{101\cdot 0}+p_{101\cdot 1}+p_{011\cdot 0},\\ 1+p_{000\cdot 0}+p_{100\cdot 0}-p_{010\cdot 1}+p_{001\cdot 0}+p_{101\cdot 0}+p_{011\cdot 0},\\ 2-p_{100\cdot 0}-p_{001\cdot 0}-p_{001\cdot 1}-p_{101\cdot 0},\\ 2-p_{000\cdot 1}-p_{100\cdot 0}-p_{100\cdot 1}-p_{001\cdot 1}-p_{101\cdot 0}-p_{101\cdot 1},\\ 2-p_{000\cdot 0}-p_{000\cdot 1}-p_{100\cdot 0}-p_{101\cdot 0},\\ 3-p_{000\cdot 0}-2p_{000\cdot 1}-2p_{100\cdot 0}-p_{100\cdot 1}-p_{001\cdot 1}-p_{101\cdot 0}-p_{101\cdot 1}\end{array}\right\}$$

Download R function for this bound (Double-click)

Back to top

## NIE$_1$-001

Lower bound =

$$\max\left\{\begin{array}{l}-p_{000\cdot 0}-p_{000\cdot 1}-p_{100\cdot 0}-p_{100\cdot 1}-p_{001\cdot 0}-p_{001\cdot 1}-p_{101\cdot 0}-p_{101\cdot 1},\\ -2+p_{000\cdot 0}+p_{000\cdot 1}+p_{100\cdot 0}+p_{100\cdot 1}+p_{001\cdot 0}+p_{001\cdot 1}+p_{101\cdot 0}+p_{101\cdot 1}\end{array}\right\}$$

Upper bound =

$$\min\left\{\begin{array}{l}2-p_{000\cdot 0}-p_{000\cdot 1}-p_{100\cdot 0}-p_{100\cdot 1}-p_{001\cdot 0}-p_{001\cdot 1}-p_{101\cdot 0}-p_{101\cdot 1},\\ p_{000\cdot 0}+p_{000\cdot 1}+p_{100\cdot 0}+p_{100\cdot 1}+p_{001\cdot 0}+p_{001\cdot 1}+p_{101\cdot 0}+p_{101\cdot 1}\end{array}\right\}$$

Download R function for this bound (Double-click)

Back to top

## $\text{NIE}_2$-001

Lower bound =

$$\max \begin{Bmatrix} -p_{000\cdot1} - p_{100\cdot0} - p_{100\cdot1} - p_{010\cdot1} - p_{110\cdot0} - p_{110\cdot1} - p_{001\cdot0} - p_{001\cdot1} - p_{101\cdot1}, \\ -p_{000\cdot1} - p_{100\cdot0} - p_{100\cdot1} - p_{010\cdot1} - p_{110\cdot0} - p_{110\cdot1} - p_{001\cdot0} - p_{011\cdot0}, \\ -1 - p_{000\cdot1} - p_{100\cdot1} + p_{010\cdot0} - p_{001\cdot1} - p_{101\cdot1} + p_{011\cdot0}, \\ -1 + p_{000\cdot0} - p_{010\cdot1} - p_{110\cdot1} - p_{001\cdot1} - p_{101\cdot1} + p_{011\cdot0}, \\ -1 - p_{001\cdot1} - p_{101\cdot1} + p_{011\cdot0}, \\ -1 - p_{100\cdot0} - p_{110\cdot0} + p_{001\cdot1} + p_{101\cdot1} - p_{011\cdot0}, \\ -2 + p_{010\cdot0} + p_{010\cdot1} + p_{110\cdot1} + p_{001\cdot0} + p_{001\cdot1} + p_{101\cdot1}, \\ -2 + p_{000\cdot0} + p_{000\cdot1} + p_{100\cdot1} + p_{001\cdot0} + p_{001\cdot1} + p_{101\cdot1}, \\ -2 + p_{000\cdot1} + p_{100\cdot1} + p_{010\cdot1} + p_{110\cdot1} + p_{001\cdot0} + p_{001\cdot1} + p_{101\cdot1}, \\ -2 + p_{100\cdot0} + p_{010\cdot0} + p_{010\cdot1} + p_{110\cdot0} + p_{110\cdot1} + p_{001\cdot0} + p_{011\cdot0}, \\ -2 + p_{000\cdot1} + p_{100\cdot0} + p_{100\cdot1} + p_{010\cdot1} + p_{110\cdot0} + p_{110\cdot1} + p_{001\cdot0} + p_{011\cdot0}, \\ -1 - p_{000\cdot1} - p_{100\cdot1} + p_{010\cdot0}, \\ -2 + p_{000\cdot0} + p_{000\cdot1} + p_{100\cdot0} + p_{100\cdot1} + p_{110\cdot0} + p_{001\cdot0} + p_{011\cdot0}, \\ -1 + p_{000\cdot0} - p_{010\cdot1} - p_{110\cdot1} \end{Bmatrix}$$

Upper bound =

$$\min \begin{Bmatrix} 1 - p_{000\cdot1} + p_{100\cdot0} - p_{100\cdot1} - p_{010\cdot1} + p_{110\cdot0} - p_{110\cdot1} + p_{001\cdot0} + p_{011\cdot0}, \\ 1 - p_{000\cdot1} - p_{100\cdot1} + p_{110\cdot0} + p_{001\cdot0} + p_{011\cdot0}, \\ 1 + p_{100\cdot0} - p_{010\cdot1} - p_{110\cdot1} + p_{001\cdot0} + p_{011\cdot0}, \\ 2 - p_{000\cdot1} - p_{100\cdot0} - p_{100\cdot1} - p_{001\cdot1} - p_{101\cdot0} - p_{101\cdot1}, \\ p_{000\cdot0} + p_{010\cdot0} + p_{010\cdot1} + p_{110\cdot0} + p_{110\cdot1} + p_{001\cdot0} + p_{001\cdot1} + p_{101\cdot0} + p_{101\cdot1} + p_{011\cdot0}, \\ 1 - p_{100\cdot0} + p_{010\cdot1} + p_{110\cdot1}, \\ 2 - p_{000\cdot1} - p_{100\cdot1} - p_{010\cdot1} - p_{110\cdot1} - p_{001\cdot1} - p_{101\cdot0} - p_{101\cdot1}, \\ p_{000\cdot0} + p_{100\cdot0} + p_{010\cdot0} + p_{110\cdot0} + p_{001\cdot0} + p_{001\cdot1} + p_{101\cdot0} + p_{101\cdot1} + p_{011\cdot0}, \\ 1 + p_{000\cdot1} - p_{100\cdot0} + p_{100\cdot1} + p_{010\cdot1} - p_{110\cdot0} + p_{110\cdot1} - p_{001\cdot0} - p_{011\cdot0}, \\ 2 - p_{100\cdot0} - p_{110\cdot0} - p_{001\cdot0} - p_{001\cdot1} - p_{101\cdot0} - p_{101\cdot1} - p_{011\cdot0}, \\ p_{000\cdot0} + p_{000\cdot1} + p_{100\cdot1} + p_{010\cdot0} + p_{010\cdot1} + p_{110\cdot1} + p_{001\cdot1} + p_{101\cdot0} + p_{101\cdot1}, \\ 2 - p_{010\cdot1} - p_{110\cdot0} - p_{110\cdot1} - p_{001\cdot1} - p_{101\cdot0} - p_{101\cdot1}, \\ p_{000\cdot0} + p_{000\cdot1} + p_{100\cdot0} + p_{100\cdot1} + p_{010\cdot0} + p_{001\cdot0} + p_{001\cdot1} + p_{101\cdot0} + p_{101\cdot1} + p_{011\cdot0}, \\ 1 + p_{000\cdot1} + p_{100\cdot1} - p_{110\cdot0} \end{Bmatrix}$$

Download R function for this bound (Double-click)

Back to top

## $\text{NIE}_{12}$-001

Lower bound =

$$\max \left\{ \begin{array}{l} -p_{000\cdot 1} - p_{100\cdot 0} - p_{100\cdot 1} - p_{010\cdot 1} - p_{110\cdot 1} - p_{001\cdot 0} - p_{001\cdot 1} - p_{101\cdot 1}, \\ -p_{000\cdot 0} - p_{000\cdot 1} - p_{100\cdot 0} - p_{100\cdot 1} - p_{001\cdot 0} - p_{001\cdot 1} - p_{101\cdot 0} - p_{101\cdot 1}, \\ -p_{000\cdot 1} - p_{100\cdot 0} - p_{100\cdot 1} - p_{010\cdot 1} - p_{110\cdot 0} - p_{110\cdot 1} - p_{001\cdot 0} - p_{011\cdot 0}, \\ -p_{000\cdot 0} - p_{000\cdot 1} - p_{100\cdot 0} - p_{100\cdot 1} - p_{110\cdot 0} - p_{001\cdot 0} - p_{101\cdot 0} - p_{011\cdot 0}, \\ -1 + p_{000\cdot 0} - p_{010\cdot 1} + p_{110\cdot 0} - p_{110\cdot 1} - p_{001\cdot 1} + p_{101\cdot 0} - p_{101\cdot 1} + p_{011\cdot 0}, \\ -1 + p_{110\cdot 0} - p_{001\cdot 1} - p_{101\cdot 1} + p_{011\cdot 0}, \\ -1 - p_{110\cdot 0} + p_{001\cdot 1} + p_{101\cdot 1} - p_{011\cdot 0}, \\ -1 - p_{000\cdot 0} + p_{010\cdot 1} - p_{110\cdot 0} + p_{110\cdot 1} + p_{001\cdot 1} - p_{101\cdot 0} + p_{101\cdot 1} - p_{011\cdot 0}, \\ -1 + p_{000\cdot 0} - p_{010\cdot 1} - p_{110\cdot 1} + p_{101\cdot 0}, \\ -2 + p_{000\cdot 0} + p_{000\cdot 1} + p_{100\cdot 0} + p_{100\cdot 1} + p_{001\cdot 0} + p_{001\cdot 1} + p_{101\cdot 0} + p_{101\cdot 1}, \\ -2 + p_{000\cdot 1} + p_{100\cdot 0} + p_{100\cdot 1} + p_{010\cdot 1} + p_{110\cdot 1} + p_{001\cdot 0} + p_{001\cdot 1} + p_{101\cdot 1}, \\ -1 - p_{000\cdot 0} + p_{010\cdot 1} + p_{110\cdot 1} - p_{101\cdot 0}, \\ -2 + p_{000\cdot 1} + p_{100\cdot 0} + p_{100\cdot 1} + p_{010\cdot 1} + p_{110\cdot 0} + p_{110\cdot 1} + p_{001\cdot 0} + p_{011\cdot 0}, \\ -2 + p_{000\cdot 0} + p_{000\cdot 1} + p_{100\cdot 0} + p_{100\cdot 1} + p_{110\cdot 0} + p_{001\cdot 0} + p_{101\cdot 0} + p_{011\cdot 0} \end{array} \right\}$$

Upper bound =

$$\min \left\{ \begin{array}{l} 2 - p_{000\cdot 0} - p_{000\cdot 1} - p_{100\cdot 1} - p_{010\cdot 1} - p_{110\cdot 1} - p_{001\cdot 1} - p_{101\cdot 0} - p_{101\cdot 1}, \\ 1 - p_{000\cdot 1} + p_{100\cdot 0} - p_{100\cdot 1} - p_{010\cdot 1} + p_{110\cdot 0} - p_{110\cdot 1} + p_{001\cdot 0} + p_{011\cdot 0}, \\ 2 - p_{000\cdot 0} - p_{000\cdot 1} - p_{100\cdot 0} - p_{100\cdot 1} - p_{001\cdot 0} - p_{001\cdot 1} - p_{101\cdot 0} - p_{101\cdot 1}, \\ 1 - p_{000\cdot 1} - p_{100\cdot 1} + p_{110\cdot 0} + p_{011\cdot 0}, \\ 2 - p_{000\cdot 0} - p_{010\cdot 1} - p_{110\cdot 0} - p_{110\cdot 1} - p_{001\cdot 1} - p_{101\cdot 0} - p_{101\cdot 1} - p_{011\cdot 0}, \\ 1 + p_{100\cdot 0} - p_{010\cdot 1} - p_{110\cdot 1} + p_{001\cdot 0}, \\ 2 - p_{000\cdot 0} - p_{100\cdot 0} - p_{110\cdot 0} - p_{001\cdot 0} - p_{001\cdot 1} - p_{101\cdot 0} - p_{101\cdot 1} - p_{011\cdot 0}, \\ p_{000\cdot 0} + p_{010\cdot 1} + p_{110\cdot 0} + p_{110\cdot 1} + p_{001\cdot 1} + p_{101\cdot 0} + p_{101\cdot 1} + p_{011\cdot 0}, \\ 1 - p_{100\cdot 0} + p_{010\cdot 1} + p_{110\cdot 1} - p_{001\cdot 0}, \\ p_{000\cdot 0} + p_{100\cdot 0} + p_{110\cdot 0} + p_{001\cdot 0} + p_{001\cdot 1} + p_{101\cdot 0} + p_{101\cdot 1} + p_{011\cdot 0}, \\ 1 + p_{000\cdot 1} - p_{100\cdot 0} + p_{100\cdot 1} + p_{010\cdot 1} - p_{110\cdot 0} + p_{110\cdot 1} - p_{001\cdot 0} - p_{011\cdot 0}, \\ p_{000\cdot 0} + p_{000\cdot 1} + p_{100\cdot 1} + p_{010\cdot 1} + p_{110\cdot 1} + p_{001\cdot 1} + p_{101\cdot 0} + p_{101\cdot 1}, \\ p_{000\cdot 0} + p_{000\cdot 1} + p_{100\cdot 0} + p_{100\cdot 1} + p_{001\cdot 0} + p_{001\cdot 1} + p_{101\cdot 0} + p_{101\cdot 1}, \\ 1 + p_{000\cdot 1} + p_{100\cdot 1} - p_{110\cdot 0} - p_{011\cdot 0} \end{array} \right\}$$

Download R function for this bound (Double-click)

Back to top

## NDE-110

Lower bound =

$$\max\left\{\begin{array}{l}-p_{000\cdot0}-2p_{000\cdot1}-p_{100\cdot0}-2p_{100\cdot1}-2p_{010\cdot1}-p_{110\cdot1}-p_{001\cdot0}-2p_{001\cdot1}-p_{101\cdot0}-2p_{101\cdot1}+p_{011\cdot0}-p_{011\cdot1},\\-3+p_{000\cdot0}+p_{100\cdot0}+p_{100\cdot1}+2p_{001\cdot0}+p_{001\cdot1}+p_{101\cdot0}+2p_{101\cdot1},\\-1-p_{000\cdot0}-p_{000\cdot1}-p_{100\cdot0}-p_{100\cdot1}+p_{010\cdot0}+p_{110\cdot1}-p_{001\cdot0}-p_{001\cdot1}-p_{101\cdot0}-p_{101\cdot1}-p_{011\cdot1},\\-3+2p_{000\cdot0}+p_{000\cdot1}+p_{100\cdot0}+2p_{100\cdot1}+p_{001\cdot0}+p_{101\cdot0}+p_{101\cdot1},\\-p_{000\cdot0}-p_{000\cdot1}-p_{100\cdot0}-p_{100\cdot1}-p_{010\cdot1}-p_{001\cdot0}-p_{001\cdot1}-p_{101\cdot0}-p_{101\cdot1}-p_{011\cdot1},\\-1-p_{000\cdot1}-p_{100\cdot1}-p_{010\cdot1}-p_{001\cdot1}-p_{101\cdot1}+p_{011\cdot0},\\-2+p_{000\cdot0}+p_{100\cdot0}+p_{100\cdot1}+p_{001\cdot0}+p_{101\cdot0}+p_{101\cdot1},\\-2+p_{100\cdot1}+p_{001\cdot0}+p_{001\cdot1}+p_{101\cdot1},\\-1-p_{000\cdot1}-p_{100\cdot1}+p_{010\cdot0}-p_{001\cdot1}-p_{101\cdot1}-p_{011\cdot1},\\-2+p_{000\cdot0}+p_{000\cdot1}+p_{100\cdot1}+p_{101\cdot1},\\-1\end{array}\right\}$$

Upper bound =

$$\min\left\{\begin{array}{l}2+p_{000\cdot0}+p_{100\cdot0}-2p_{010\cdot1}-p_{110\cdot0}-p_{110\cdot1}+p_{001\cdot0}+p_{101\cdot0}-p_{011\cdot1},\\3-p_{000\cdot0}-p_{000\cdot1}-p_{100\cdot0}-p_{001\cdot0}-2p_{001\cdot1}-2p_{101\cdot0}-p_{101\cdot1},\\2p_{000\cdot0}+p_{000\cdot1}+2p_{100\cdot0}+p_{100\cdot1}+p_{010\cdot0}+p_{110\cdot0}+p_{110\cdot1}+2p_{001\cdot0}+p_{001\cdot1}+2p_{101\cdot0}+p_{101\cdot1}+p_{011\cdot0}-p_{011\cdot1},\\1,\\2-p_{010\cdot1}-p_{110\cdot0}-p_{110\cdot1}-p_{011\cdot1},\\p_{000\cdot0}+p_{000\cdot1}+p_{100\cdot0}+p_{100\cdot1}+p_{010\cdot0}+p_{110\cdot0}+p_{110\cdot1}+p_{001\cdot0}+p_{001\cdot1}+p_{101\cdot0}+p_{101\cdot1}+p_{011\cdot0},\\1+p_{000\cdot0}+p_{100\cdot0}-p_{010\cdot1}+p_{001\cdot0}+p_{101\cdot0}-p_{011\cdot1},\\2-p_{000\cdot1}-p_{100\cdot0}-p_{100\cdot1}-p_{001\cdot1},\\2-p_{000\cdot1}-p_{001\cdot1}-p_{101\cdot0}-p_{101\cdot1},\\2-p_{000\cdot0}-p_{000\cdot1}-p_{100\cdot0}-p_{001\cdot0}-p_{001\cdot1}-p_{101\cdot0},\\3-p_{000\cdot0}-2p_{000\cdot1}-2p_{100\cdot0}-p_{100\cdot1}-p_{001\cdot0}-p_{001\cdot1}-p_{101\cdot0}\end{array}\right\}$$

Download R function for this bound (Double-click)

Back to top

## NIE$_1$-110

Lower bound =

$$\max\left\{\begin{array}{l}-p_{000\cdot0}-p_{000\cdot1}-p_{100\cdot0}-p_{100\cdot1}-p_{001\cdot0}-p_{001\cdot1}-p_{101\cdot0}-p_{101\cdot1},\\-2+p_{000\cdot0}+p_{000\cdot1}+p_{100\cdot0}+p_{100\cdot1}+p_{001\cdot0}+p_{001\cdot1}+p_{101\cdot0}+p_{101\cdot1}\end{array}\right\}$$

Upper bound =

$$\min\left\{\begin{array}{l}2-p_{000\cdot0}-p_{000\cdot1}-p_{100\cdot0}-p_{100\cdot1}-p_{001\cdot0}-p_{001\cdot1}-p_{101\cdot0}-p_{101\cdot1},\\p_{000\cdot0}+p_{000\cdot1}+p_{100\cdot0}+p_{100\cdot1}+p_{001\cdot0}+p_{001\cdot1}+p_{101\cdot0}+p_{101\cdot1}\end{array}\right\}$$

Download R function for this bound (Double-click)

Back to top

## NIE$_2$-110

Lower bound =

$$\max\left\{\begin{array}{l}-p_{000\cdot0}-p_{000\cdot1}-p_{100\cdot0}-p_{010\cdot0}-p_{010\cdot1}-p_{110\cdot0}-p_{001\cdot0}-p_{101\cdot0}-p_{101\cdot1},\\ -p_{000\cdot0}-p_{000\cdot1}-p_{100\cdot0}-p_{100\cdot1}-p_{010\cdot1}-p_{001\cdot0}-p_{001\cdot1}-p_{101\cdot0}-p_{101\cdot1}-p_{011\cdot1},\\ -p_{000\cdot1}-p_{010\cdot0}-p_{010\cdot1}-p_{110\cdot0}-p_{110\cdot1}-p_{001\cdot0}-p_{001\cdot1}-p_{101\cdot0}-p_{101\cdot1}-p_{011\cdot1},\\ -p_{000\cdot1}-p_{100\cdot1}-p_{010\cdot1}-p_{110\cdot1}-p_{001\cdot0}-p_{001\cdot1}-p_{101\cdot0}-p_{101\cdot1}-p_{011\cdot1},\\ -1-p_{000\cdot0}-p_{100\cdot0}+p_{100\cdot1}-p_{010\cdot0}-p_{110\cdot0}+p_{110\cdot1}+p_{001\cdot1}+p_{011\cdot1},\\ -2+p_{100\cdot1}+p_{110\cdot1}+p_{001\cdot0}+p_{001\cdot1}+p_{101\cdot0}+p_{101\cdot1}+p_{011\cdot1},\\ -2+p_{010\cdot0}+p_{110\cdot0}+p_{110\cdot1}+p_{001\cdot0}+p_{101\cdot0}+p_{101\cdot1},\\ -2+p_{000\cdot0}+p_{100\cdot0}+p_{100\cdot1}+p_{001\cdot0}+p_{101\cdot0}+p_{101\cdot1},\\ -2+p_{000\cdot0}+p_{100\cdot0}+p_{010\cdot0}+p_{110\cdot0}+p_{001\cdot0}+p_{101\cdot0}+p_{101\cdot1},\\ -1-p_{000\cdot0}-p_{100\cdot0}+p_{110\cdot1},\\ -1-p_{100\cdot1}+p_{010\cdot0}+p_{110\cdot0}-p_{001\cdot1}-p_{011\cdot1},\\ -1+p_{000\cdot0}+p_{100\cdot0}-p_{100\cdot1}+p_{010\cdot0}+p_{110\cdot0}-p_{110\cdot1}-p_{001\cdot1}-p_{011\cdot1},\\ -1+p_{100\cdot1}-p_{010\cdot0}-p_{110\cdot0},\\ -1+p_{000\cdot0}+p_{100\cdot0}-p_{110\cdot1}-p_{001\cdot1}-p_{011\cdot1}\end{array}\right\}$$

Upper bound =

$$\min\left\{\begin{array}{l}2-p_{000\cdot0}-p_{000\cdot1}-p_{100\cdot0}-p_{100\cdot1}-p_{110\cdot1}-p_{001\cdot1}-p_{011\cdot1},\\ 2-p_{000\cdot0}-p_{000\cdot1}-p_{100\cdot0}-p_{001\cdot0}-p_{001\cdot1}-p_{101\cdot0},\\ 1-p_{000\cdot1}+p_{010\cdot0}+p_{110\cdot0}+p_{001\cdot0}+p_{101\cdot0}-p_{011\cdot1},\\ 1-p_{000\cdot1}+p_{010\cdot0}+p_{110\cdot0},\\ 2-p_{000\cdot0}-p_{100\cdot0}-p_{100\cdot1}-p_{010\cdot0}-p_{110\cdot0}-p_{110\cdot1}-p_{001\cdot1}-p_{011\cdot1},\\ 2-p_{000\cdot0}-p_{100\cdot0}-p_{010\cdot0}-p_{110\cdot0}-p_{001\cdot0}-p_{001\cdot1}-p_{101\cdot0},\\ 1+p_{001\cdot0}+p_{101\cdot0}-p_{011\cdot1},\\ p_{000\cdot0}+p_{100\cdot0}+p_{100\cdot1}+p_{010\cdot0}+p_{110\cdot0}+p_{110\cdot1}+p_{001\cdot1}+p_{011\cdot1},\\ 1+p_{100\cdot1}+p_{110\cdot1}-p_{001\cdot0}-p_{101\cdot0}+p_{011\cdot1},\\ p_{000\cdot0}+p_{100\cdot0}+p_{100\cdot1}+p_{010\cdot0}+p_{110\cdot0}+p_{110\cdot1}+p_{001\cdot0}+p_{001\cdot1}+p_{101\cdot0},\\ 2-p_{100\cdot1}-p_{010\cdot0}-p_{010\cdot1}-p_{110\cdot0}-p_{110\cdot1}-p_{001\cdot1}-p_{011\cdot1},\\ 2-p_{010\cdot0}-p_{010\cdot1}-p_{110\cdot0}-p_{001\cdot0}-p_{001\cdot1}-p_{101\cdot0},\\ 1+p_{000\cdot0}+p_{100\cdot0}-p_{010\cdot1}+p_{001\cdot0}+p_{101\cdot0}-p_{011\cdot1},\\ 1+p_{000\cdot0}+p_{100\cdot0}-p_{010\cdot1}\end{array}\right\}$$

Download R function for this bound (Double-click)

Back to top

## $\mathbf{NIE_{12}}$-110

Lower bound =

$$\max\left\{\begin{array}{l}
-p_{000\cdot0} - p_{000\cdot1} - p_{100\cdot0} - p_{010\cdot0} - p_{110\cdot0} - p_{001\cdot0} - p_{101\cdot0} - p_{101\cdot1},\\
-p_{000\cdot0} - p_{000\cdot1} - p_{100\cdot0} - p_{100\cdot1} - p_{001\cdot0} - p_{001\cdot1} - p_{101\cdot0} - p_{101\cdot1},\\
-p_{000\cdot1} - p_{010\cdot0} - p_{110\cdot0} - p_{110\cdot1} - p_{001\cdot0} - p_{101\cdot0} - p_{101\cdot1} - p_{011\cdot1},\\
-p_{000\cdot1} - p_{100\cdot1} - p_{110\cdot1} - p_{001\cdot0} - p_{001\cdot1} - p_{101\cdot0} - p_{101\cdot1} - p_{011\cdot1},\\
-1 - p_{000\cdot0} - p_{100\cdot0} + p_{100\cdot1} - p_{010\cdot0} - p_{110\cdot0} + p_{110\cdot1} + p_{001\cdot1} + p_{011\cdot1},\\
-1 - p_{000\cdot0} - p_{100\cdot0} + p_{110\cdot1} + p_{011\cdot1},\\
-2 + p_{000\cdot1} + p_{100\cdot1} + p_{110\cdot1} + p_{001\cdot0} + p_{001\cdot1} + p_{101\cdot0} + p_{101\cdot1} + p_{011\cdot1},\\
-2 + p_{000\cdot1} + p_{010\cdot0} + p_{110\cdot0} + p_{110\cdot1} + p_{001\cdot0} + p_{101\cdot0} + p_{101\cdot1} + p_{011\cdot1},\\
-2 + p_{000\cdot0} + p_{000\cdot1} + p_{100\cdot0} + p_{100\cdot1} + p_{001\cdot0} + p_{001\cdot1} + p_{101\cdot0} + p_{101\cdot1},\\
-2 + p_{000\cdot0} + p_{000\cdot1} + p_{100\cdot0} + p_{010\cdot0} + p_{110\cdot0} + p_{001\cdot0} + p_{101\cdot0} + p_{101\cdot1},\\
-1 + p_{100\cdot1} - p_{010\cdot0} - p_{110\cdot0} + p_{001\cdot1},\\
-1 - p_{100\cdot1} + p_{010\cdot0} + p_{110\cdot0} - p_{001\cdot1},\\
-1 + p_{000\cdot0} + p_{100\cdot0} - p_{100\cdot1} + p_{010\cdot0} + p_{110\cdot0} - p_{110\cdot1} - p_{001\cdot1} - p_{011\cdot1},\\
-1 + p_{000\cdot0} + p_{100\cdot0} - p_{110\cdot1} - p_{011\cdot1}
\end{array}\right\}$$

Upper bound =

$$\min\left\{\begin{array}{l}
2 - p_{000\cdot0} - p_{000\cdot1} - p_{100\cdot0} - p_{100\cdot1} - p_{110\cdot1} - p_{001\cdot1} - p_{101\cdot1} - p_{011\cdot1},\\
2 - p_{000\cdot0} - p_{000\cdot1} - p_{100\cdot0} - p_{100\cdot1} - p_{001\cdot0} - p_{001\cdot1} - p_{101\cdot0} - p_{101\cdot1},\\
1 - p_{000\cdot1} + p_{010\cdot0} + p_{110\cdot0} - p_{110\cdot1} + p_{001\cdot0} + p_{101\cdot0} - p_{101\cdot1} - p_{011\cdot1},\\
1 - p_{000\cdot1} + p_{010\cdot0} + p_{110\cdot0} - p_{101\cdot1},\\
2 - p_{000\cdot0} - p_{100\cdot0} - p_{100\cdot1} - p_{010\cdot0} - p_{110\cdot0} - p_{110\cdot1} - p_{001\cdot1} - p_{011\cdot1},\\
2 - p_{000\cdot0} - p_{100\cdot0} - p_{100\cdot1} - p_{010\cdot0} - p_{110\cdot0} - p_{001\cdot0} - p_{001\cdot1} - p_{101\cdot0},\\
1 - p_{110\cdot1} + p_{001\cdot0} + p_{101\cdot0} - p_{011\cdot1},\\
p_{000\cdot0} + p_{100\cdot0} + p_{100\cdot1} + p_{010\cdot0} + p_{110\cdot0} + p_{110\cdot1} + p_{001\cdot1} + p_{011\cdot1},\\
1 + p_{110\cdot1} - p_{001\cdot0} - p_{101\cdot0} + p_{011\cdot1},\\
p_{000\cdot0} + p_{100\cdot0} + p_{100\cdot1} + p_{010\cdot0} + p_{110\cdot0} + p_{001\cdot0} + p_{001\cdot1} + p_{101\cdot0},\\
1 + p_{000\cdot1} - p_{010\cdot0} - p_{110\cdot0} + p_{110\cdot1} - p_{001\cdot0} - p_{101\cdot0} + p_{101\cdot1} + p_{011\cdot1},\\
1 + p_{000\cdot1} - p_{010\cdot0} - p_{110\cdot0} + p_{101\cdot1},\\
p_{000\cdot0} + p_{000\cdot1} + p_{100\cdot0} + p_{100\cdot1} + p_{001\cdot0} + p_{001\cdot1} + p_{101\cdot0} + p_{101\cdot1},\\
p_{000\cdot0} + p_{000\cdot1} + p_{100\cdot0} + p_{100\cdot1} + p_{110\cdot1} + p_{001\cdot1} + p_{101\cdot1} + p_{011\cdot1}
\end{array}\right\}$$

Download R function for this bound (Double-click)

Back to top

## NDE-101

Lower bound =

$$\max \begin{Bmatrix} -p_{000\cdot0} - 2p_{000\cdot1} - p_{100\cdot0} - 2p_{100\cdot1} - p_{010\cdot1} - p_{110\cdot0} - p_{110\cdot1} - p_{001\cdot0} - 2p_{001\cdot1} - p_{101\cdot0} - 2p_{101\cdot1} + p_{011\cdot0} - p_{011\cdot1}, \\ -3 + p_{000\cdot0} + p_{000\cdot1} + p_{100\cdot1} + 2p_{001\cdot0} + p_{001\cdot1} + p_{101\cdot0} + 2p_{101\cdot1}, \\ -2 - p_{000\cdot1} - p_{100\cdot1} + 2p_{010\cdot0} + p_{110\cdot0} + p_{110\cdot1} - p_{001\cdot1} - p_{101\cdot1} + p_{011\cdot0}, \\ -3 + 2p_{000\cdot0} + p_{000\cdot1} + p_{100\cdot0} + 2p_{100\cdot1} + p_{001\cdot0} + p_{001\cdot1} + p_{101\cdot1}, \\ -p_{000\cdot0} - p_{000\cdot1} - p_{100\cdot0} - p_{100\cdot1} - p_{010\cdot1} - p_{110\cdot0} - p_{110\cdot1} - p_{001\cdot0} - p_{001\cdot1} - p_{101\cdot0} - p_{101\cdot1} - p_{011\cdot1}, \\ -1 - p_{000\cdot1} - p_{100\cdot1} + p_{010\cdot0} - p_{001\cdot1} - p_{101\cdot1} + p_{011\cdot0}, \\ -2 + p_{000\cdot0} + p_{001\cdot0} + p_{101\cdot0} + p_{101\cdot1}, \\ -2 + p_{000\cdot0} + p_{000\cdot1} + p_{100\cdot1} + p_{001\cdot0} + p_{001\cdot1} + p_{101\cdot1}, \\ -2 + p_{010\cdot0} + p_{110\cdot0} + p_{110\cdot1} + p_{011\cdot0}, \\ -2 + p_{000\cdot0} + p_{100\cdot0} + p_{100\cdot1} + p_{001\cdot0}, \\ -1 \end{Bmatrix}$$

Upper bound =

$$\min \begin{Bmatrix} 1 + p_{000\cdot0} + p_{000\cdot1} + p_{100\cdot0} + p_{100\cdot1} - p_{010\cdot1} - p_{110\cdot0} + p_{001\cdot0} + p_{001\cdot1} + p_{101\cdot0} + p_{101\cdot1} + p_{011\cdot0}, \\ 3 - p_{000\cdot1} - p_{100\cdot0} - p_{100\cdot1} - p_{001\cdot0} - 2p_{001\cdot1} - 2p_{101\cdot0} - p_{101\cdot1}, \\ 2p_{000\cdot0} + p_{000\cdot1} + 2p_{100\cdot0} + p_{100\cdot1} + 2p_{010\cdot0} + p_{110\cdot0} + 2p_{001\cdot0} + p_{001\cdot1} + 2p_{101\cdot0} + p_{101\cdot1} + p_{011\cdot0} - p_{011\cdot1}, \\ 1, \\ 1 + p_{000\cdot0} + p_{100\cdot0} + p_{010\cdot0} + p_{001\cdot0} + p_{101\cdot0} - p_{011\cdot1}, \\ p_{000\cdot0} + p_{000\cdot1} + p_{100\cdot0} + p_{100\cdot1} + p_{010\cdot0} + p_{001\cdot0} + p_{001\cdot1} + p_{101\cdot0} + p_{101\cdot1} + p_{011\cdot0}, \\ 1 + p_{000\cdot0} + p_{100\cdot0} - p_{010\cdot1} + p_{001\cdot0} + p_{101\cdot0} + p_{011\cdot0}, \\ 2 - p_{100\cdot0} - p_{001\cdot0} - p_{001\cdot1} - p_{101\cdot0}, \\ 2 - p_{000\cdot1} - p_{100\cdot0} - p_{100\cdot1} - p_{001\cdot1} - p_{101\cdot0} - p_{101\cdot1}, \\ 2 - p_{000\cdot0} - p_{000\cdot1} - p_{100\cdot0} - p_{101\cdot0}, \\ 3 - p_{000\cdot0} - 2p_{000\cdot1} - 2p_{100\cdot0} - p_{100\cdot1} - p_{001\cdot1} - p_{101\cdot0} - p_{101\cdot1} \end{Bmatrix}$$

Download R function for this bound (Double-click)

Back to top

## NIE$_1$-101

Lower bound =

$$\max \begin{Bmatrix} -p_{000\cdot0} - p_{000\cdot1} - p_{100\cdot0} - p_{100\cdot1} - p_{001\cdot0} - p_{001\cdot1} - p_{101\cdot0} - p_{101\cdot1}, \\ -2 + p_{000\cdot0} + p_{000\cdot1} + p_{100\cdot0} + p_{100\cdot1} + p_{001\cdot0} + p_{001\cdot1} + p_{101\cdot0} + p_{101\cdot1} \end{Bmatrix}$$

Upper bound =

$$\min \begin{Bmatrix} 2 - p_{000\cdot0} - p_{000\cdot1} - p_{100\cdot0} - p_{100\cdot1} - p_{001\cdot0} - p_{001\cdot1} - p_{101\cdot0} - p_{101\cdot1}, \\ p_{000\cdot0} + p_{000\cdot1} + p_{100\cdot0} + p_{100\cdot1} + p_{001\cdot0} + p_{001\cdot1} + p_{101\cdot0} + p_{101\cdot1} \end{Bmatrix}$$

Download R function for this bound (Double-click)

Back to top

## NIE$_2$-101

Lower bound =

$$\max\left\{\begin{array}{l}-p_{000\cdot 0}-p_{000\cdot 1}-p_{100\cdot 0}-p_{100\cdot 1}-p_{010\cdot 0}-p_{010\cdot 1}-p_{110\cdot 0}-p_{001\cdot 0}-p_{001\cdot 1}-p_{101\cdot 0}-p_{101\cdot 1},\\ -p_{000\cdot 0}-p_{000\cdot 1}-p_{100\cdot 0}-p_{100\cdot 1}-p_{010\cdot 1}-p_{001\cdot 0}-p_{001\cdot 1}-p_{101\cdot 0}-p_{101\cdot 1}-p_{011\cdot 1},\\ -2+p_{100\cdot 1}+p_{001\cdot 0}+p_{001\cdot 1}+p_{101\cdot 0}+p_{101\cdot 1},\\ -2+p_{000\cdot 0}+p_{100\cdot 0}+p_{100\cdot 1}+p_{001\cdot 0}+p_{101\cdot 0}+p_{101\cdot 1},\\ -1-p_{000\cdot 1}-p_{100\cdot 1}+p_{010\cdot 0}+p_{110\cdot 0}-p_{001\cdot 1}-p_{101\cdot 1}-p_{011\cdot 1},\\ -2+p_{000\cdot 0}+p_{000\cdot 1}+p_{100\cdot 0}+p_{100\cdot 1}+p_{101\cdot 1},\\ -1\end{array}\right\}$$

Upper bound =

$$\min\left\{\begin{array}{l}2-p_{000\cdot 0}-p_{000\cdot 1}-p_{100\cdot 0}-p_{100\cdot 1}-p_{001\cdot 1},\\ 2-p_{000\cdot 0}-p_{000\cdot 1}-p_{100\cdot 0}-p_{001\cdot 0}-p_{001\cdot 1}-p_{101\cdot 0},\\ 2-p_{000\cdot 1}-p_{001\cdot 0}-p_{001\cdot 1}-p_{101\cdot 0}-p_{101\cdot 1},\\ 2-p_{010\cdot 0}-p_{010\cdot 1}-p_{110\cdot 0}-p_{110\cdot 1}-p_{011\cdot 1},\\ 1+p_{000\cdot 0}+p_{100\cdot 0}-p_{010\cdot 1}+p_{001\cdot 0}+p_{101\cdot 0}-p_{011\cdot 1},\\ p_{000\cdot 0}+p_{000\cdot 1}+p_{100\cdot 0}+p_{100\cdot 1}+p_{010\cdot 0}+p_{110\cdot 0}+p_{110\cdot 1}+p_{001\cdot 0}+p_{001\cdot 1}+p_{101\cdot 0}+p_{101\cdot 1},\\ 1\end{array}\right\}$$

Download R function for this bound (Double-click)

Back to top

## NIE$_{12}$-101

Lower bound =

$$\max\left\{\begin{array}{l}-p_{000\cdot 0}-p_{000\cdot 1}-p_{100\cdot 0}-p_{100\cdot 1}-p_{001\cdot 0}-p_{001\cdot 1}-p_{101\cdot 0}-p_{101\cdot 1},\\ -2+p_{000\cdot 0}+p_{000\cdot 1}+p_{100\cdot 0}+p_{100\cdot 1}+p_{001\cdot 0}+p_{001\cdot 1}+p_{101\cdot 0}+p_{101\cdot 1}\end{array}\right\}$$

Upper bound =

$$\min\left\{\begin{array}{l}2-p_{000\cdot 0}-p_{000\cdot 1}-p_{100\cdot 0}-p_{100\cdot 1}-p_{001\cdot 0}-p_{001\cdot 1}-p_{101\cdot 0}-p_{101\cdot 1},\\ p_{000\cdot 0}+p_{000\cdot 1}+p_{100\cdot 0}+p_{100\cdot 1}+p_{001\cdot 0}+p_{001\cdot 1}+p_{101\cdot 0}+p_{101\cdot 1}\end{array}\right\}$$

Download R function for this bound (Double-click)

Back to top

## NDE-011

Lower bound =

$$\max \begin{Bmatrix} -p_{000\cdot 0} - 2p_{000\cdot 1} - p_{100\cdot 0} - 2p_{100\cdot 1} - 2p_{010\cdot 1} - p_{110\cdot 1} - p_{001\cdot 1} - p_{101\cdot 0} - p_{101\cdot 1} + p_{011\cdot 0} - p_{011\cdot 1}, \\ -2 + p_{000\cdot 0} - p_{000\cdot 1} + p_{100\cdot 0} - p_{010\cdot 1} - p_{110\cdot 1} + 2p_{001\cdot 0} + p_{101\cdot 0} + p_{101\cdot 1} + p_{011\cdot 0}, \\ -1 - p_{100\cdot 0} + p_{010\cdot 0} + p_{110\cdot 1} - p_{001\cdot 0} - p_{001\cdot 1} - p_{101\cdot 0} - p_{101\cdot 1} - p_{011\cdot 1}, \\ -3 + 2p_{000\cdot 0} + p_{000\cdot 1} + p_{100\cdot 0} + 2p_{100\cdot 1} + p_{010\cdot 0} + p_{010\cdot 1} + p_{110\cdot 1} + p_{001\cdot 0} + p_{101\cdot 0} + p_{101\cdot 1}, \\ -p_{000\cdot 0} - p_{000\cdot 1} - p_{100\cdot 0} - p_{100\cdot 1} - p_{010\cdot 1} - p_{110\cdot 1} - p_{001\cdot 1} - p_{101\cdot 0} - p_{101\cdot 1} - p_{011\cdot 1}, \\ -p_{000\cdot 0} - p_{000\cdot 1} - p_{100\cdot 0} - p_{100\cdot 1} - p_{010\cdot 1} - p_{001\cdot 0} - p_{001\cdot 1} - p_{101\cdot 0} - p_{101\cdot 1} - p_{011\cdot 1}, \\ -1 - p_{000\cdot 1} - p_{100\cdot 1} - p_{010\cdot 1} - p_{110\cdot 1} + p_{001\cdot 0} + p_{011\cdot 0}, \\ -1 - p_{000\cdot 1} - p_{100\cdot 1} - p_{010\cdot 1} + p_{011\cdot 0}, \\ -2 + p_{000\cdot 0} + p_{100\cdot 0} + p_{001\cdot 0} + p_{101\cdot 0} + p_{101\cdot 1} + p_{011\cdot 0}, \\ -2 + p_{000\cdot 0} + p_{110\cdot 1} + p_{101\cdot 1} + p_{011\cdot 0}, \\ -2 + p_{000\cdot 0} + p_{100\cdot 0} + p_{100\cdot 1} + p_{001\cdot 0} + p_{101\cdot 0} + p_{101\cdot 1}, \\ -1 - p_{000\cdot 1} - p_{010\cdot 1} - p_{110\cdot 1} + p_{001\cdot 0}, \\ -1 - p_{000\cdot 1} + p_{010\cdot 0} - p_{010\cdot 1} - p_{110\cdot 1} + p_{001\cdot 0} - p_{001\cdot 1} - p_{101\cdot 1} - p_{011\cdot 1}, \\ -1 - p_{100\cdot 0} + p_{110\cdot 1} - p_{001\cdot 0} - p_{101\cdot 0}, \\ -1 + p_{010\cdot 0} - p_{001\cdot 1} - p_{101\cdot 1} - p_{011\cdot 1}, \\ -2 + p_{000\cdot 0} + p_{000\cdot 1} + p_{100\cdot 1} + p_{010\cdot 0} + p_{010\cdot 1} + p_{110\cdot 1}, \\ -2 + p_{000\cdot 0} + p_{100\cdot 0} + p_{100\cdot 1} + p_{010\cdot 0} + p_{001\cdot 0} + p_{101\cdot 0}, \\ -2 + p_{000\cdot 0} + p_{000\cdot 1} + p_{100\cdot 1} + p_{010\cdot 1} + p_{110\cdot 1} + p_{101\cdot 1}, \\ -1 \end{Bmatrix}$$

Upper bound =

$$\min\left\{\begin{array}{l}
2+p_{000\cdot 0}-p_{000\cdot 1}-p_{100\cdot 1}-2p_{010\cdot 1}-p_{110\cdot 0}-p_{110\cdot 1}+p_{001\cdot 0}+p_{101\cdot 0}-p_{011\cdot 1},\\
1+p_{100\cdot 1}+p_{010\cdot 0}+p_{010\cdot 1}+p_{110\cdot 0}+p_{110\cdot 1}-p_{001\cdot 1}-p_{101\cdot 0}+p_{011\cdot 0},\\
2p_{000\cdot 0}+p_{000\cdot 1}+2p_{100\cdot 0}+p_{100\cdot 1}+p_{010\cdot 0}+p_{110\cdot 0}+p_{110\cdot 1}+2p_{001\cdot 0}+p_{101\cdot 0}+p_{011\cdot 0}-p_{011\cdot 1},\\
1,\\
p_{000\cdot 0}+p_{000\cdot 1}+p_{100\cdot 0}+p_{100\cdot 1}+p_{010\cdot 0}+p_{010\cdot 1}+p_{110\cdot 0}+p_{110\cdot 1}+p_{001\cdot 0}+p_{011\cdot 0},\\
p_{000\cdot 0}+p_{000\cdot 1}+p_{100\cdot 0}+p_{100\cdot 1}+p_{010\cdot 0}+p_{110\cdot 0}+p_{110\cdot 1}+p_{001\cdot 0}+p_{101\cdot 0}+p_{011\cdot 0},\\
1+p_{000\cdot 0}+p_{100\cdot 0}+p_{001\cdot 0}-p_{011\cdot 1},\\
1+p_{000\cdot 0}+p_{100\cdot 0}-p_{010\cdot 1}+p_{001\cdot 0}+p_{101\cdot 0}-p_{011\cdot 1},\\
1+p_{000\cdot 0}-p_{010\cdot 1}+p_{001\cdot 0}+p_{101\cdot 0},\\
1+p_{000\cdot 0}+p_{010\cdot 0}-p_{010\cdot 1}+p_{110\cdot 0}+p_{001\cdot 0}-p_{001\cdot 1}+p_{101\cdot 0}+p_{011\cdot 0},\\
2-p_{000\cdot 1}-p_{100\cdot 0}-p_{100\cdot 1}-p_{010\cdot 1}-p_{110\cdot 1}-p_{001\cdot 1},\\
1+p_{100\cdot 1}+p_{010\cdot 1}+p_{110\cdot 1}-p_{101\cdot 0},\\
2-p_{000\cdot 1}-p_{100\cdot 1}-p_{010\cdot 1}-p_{110\cdot 0}-p_{110\cdot 1}-p_{011\cdot 1},\\
2-p_{000\cdot 1}-p_{100\cdot 0}-p_{100\cdot 1}-p_{010\cdot 1}-p_{110\cdot 0}-p_{110\cdot 1},\\
2-p_{000\cdot 1}-p_{110\cdot 0}-p_{101\cdot 0}-p_{011\cdot 1},\\
1+p_{010\cdot 0}+p_{110\cdot 0}-p_{001\cdot 1}+p_{011\cdot 0},\\
2-p_{000\cdot 0}-p_{000\cdot 1}-p_{100\cdot 0}-p_{110\cdot 0}-p_{001\cdot 0}-p_{101\cdot 0},\\
2-p_{000\cdot 0}-p_{000\cdot 1}-p_{100\cdot 0}-p_{001\cdot 0}-p_{001\cdot 1}-p_{101\cdot 0},\\
3-p_{000\cdot 0}-2p_{000\cdot 1}-2p_{100\cdot 0}-p_{100\cdot 1}-p_{010\cdot 1}-p_{110\cdot 0}-p_{110\cdot 1}-p_{001\cdot 0}-p_{001\cdot 1}-p_{101\cdot 0}
\end{array}\right\}$$

Download R function for this bound (Double-click)

Back to top

## $\mathbf{NIE_1}$-011

Lower bound =

$$\max\left\{\begin{array}{l}
-p_{000\cdot0} - p_{000\cdot1} - p_{100\cdot0} - p_{100\cdot1} - p_{010\cdot1} - p_{110\cdot1} - p_{001\cdot1} - p_{101\cdot0} - p_{101\cdot1},\\
-p_{000\cdot0} - p_{000\cdot1} - p_{100\cdot0} - p_{100\cdot1} - p_{001\cdot0} - p_{001\cdot1} - p_{101\cdot0} - p_{101\cdot1},\\
-1 - p_{000\cdot1} - p_{100\cdot1} - p_{010\cdot1} - p_{110\cdot1} + p_{001\cdot0} + p_{011\cdot0},\\
-1 - p_{000\cdot1} - p_{100\cdot1} + p_{011\cdot0},\\
-2 + p_{000\cdot0} + p_{100\cdot0} + p_{001\cdot0} + p_{001\cdot1} + p_{101\cdot0} + p_{101\cdot1} + p_{011\cdot0},\\
-2 + p_{000\cdot0} + p_{010\cdot1} + p_{110\cdot1} + p_{001\cdot1} + p_{101\cdot1} + p_{011\cdot0},\\
-2 + p_{000\cdot0} + p_{000\cdot1} + p_{100\cdot0} + p_{100\cdot1} + p_{001\cdot0} + p_{001\cdot1} + p_{101\cdot0} + p_{101\cdot1},\\
-1 + p_{010\cdot0} - p_{010\cdot1} - p_{110\cdot1} + p_{001\cdot0} - p_{001\cdot1} - p_{101\cdot1},\\
-1 - p_{010\cdot1} - p_{110\cdot1} + p_{001\cdot0},\\
-1 - p_{100\cdot0} + p_{010\cdot1} + p_{110\cdot1} - p_{001\cdot0} - p_{101\cdot0},\\
-1 + p_{010\cdot0} - p_{001\cdot1} - p_{101\cdot1},\\
-2 + p_{000\cdot0} + p_{000\cdot1} + p_{100\cdot1} + p_{010\cdot0} + p_{010\cdot1} + p_{110\cdot1},\\
-2 + p_{000\cdot0} + p_{000\cdot1} + p_{100\cdot0} + p_{100\cdot1} + p_{010\cdot0} + p_{001\cdot0} + p_{101\cdot0},\\
-2 + p_{000\cdot0} + p_{000\cdot1} + p_{100\cdot1} + p_{010\cdot1} + p_{110\cdot1} + p_{001\cdot1} + p_{101\cdot1}
\end{array}\right\}$$

Upper bound =

$$\min\left\{\begin{array}{l}
2 - p_{000\cdot0} - p_{000\cdot1} - p_{100\cdot0} - p_{100\cdot1} - p_{001\cdot0} - p_{001\cdot1} - p_{101\cdot0} - p_{101\cdot1},\\
2 - p_{000\cdot0} - p_{000\cdot1} - p_{100\cdot0} - p_{100\cdot1} - p_{110\cdot0} - p_{001\cdot0} - p_{101\cdot0},\\
1 + p_{010\cdot0} + p_{110\cdot0} - p_{001\cdot1} - p_{101\cdot1} + p_{011\cdot0},\\
2 - p_{000\cdot1} - p_{100\cdot0} - p_{100\cdot1} - p_{010\cdot1} - p_{110\cdot0} - p_{110\cdot1},\\
2 - p_{000\cdot1} - p_{100\cdot0} - p_{100\cdot1} - p_{010\cdot1} - p_{110\cdot1} - p_{001\cdot1} - p_{101\cdot1},\\
1 + p_{010\cdot1} - p_{110\cdot0} + p_{110\cdot1} + p_{001\cdot1} - p_{101\cdot0} + p_{101\cdot1},\\
1 - p_{110\cdot0} + p_{001\cdot1} + p_{101\cdot1},\\
1 + p_{010\cdot1} + p_{110\cdot1} - p_{101\cdot0},\\
1 + p_{000\cdot0} + p_{010\cdot0} - p_{010\cdot1} + p_{110\cdot0} - p_{110\cdot1} + p_{001\cdot0} - p_{001\cdot1} + p_{101\cdot0} - p_{101\cdot1} + p_{011\cdot0},\\
1 + p_{000\cdot0} - p_{010\cdot1} - p_{110\cdot1} + p_{001\cdot0} + p_{101\cdot0},\\
p_{000\cdot0} + p_{000\cdot1} + p_{100\cdot0} + p_{100\cdot1} + p_{001\cdot0} + p_{001\cdot1} + p_{101\cdot0} + p_{101\cdot1},\\
p_{000\cdot0} + p_{000\cdot1} + p_{100\cdot0} + p_{100\cdot1} + p_{010\cdot1} + p_{110\cdot1} + p_{001\cdot0} + p_{001\cdot1} + p_{101\cdot1},\\
p_{000\cdot0} + p_{000\cdot1} + p_{100\cdot0} + p_{100\cdot1} + p_{010\cdot0} + p_{110\cdot0} + p_{001\cdot0} + p_{101\cdot0} + p_{011\cdot0},\\
p_{000\cdot0} + p_{000\cdot1} + p_{100\cdot0} + p_{100\cdot1} + p_{010\cdot0} + p_{010\cdot1} + p_{110\cdot0} + p_{110\cdot1} + p_{001\cdot0} + p_{011\cdot0}
\end{array}\right\}$$

Download R function for this bound (Double-click)

Back to top

## $\mathbf{NIE_2}$-011

Lower bound =

$$\max\left\{\begin{array}{l}-p_{000\cdot0}-p_{000\cdot1}-p_{100\cdot0}-p_{100\cdot1}-p_{010\cdot1}-p_{110\cdot0}-p_{110\cdot1}-p_{001\cdot0}-p_{001\cdot1}-p_{101\cdot0}-p_{101\cdot1},\\ -1-p_{000\cdot1}-p_{100\cdot1}+p_{010\cdot0}-p_{001\cdot1}-p_{101\cdot1}+p_{011\cdot0},\\ -2+p_{000\cdot0}+p_{001\cdot0}+p_{001\cdot1}+p_{101\cdot0}+p_{101\cdot1},\\ -2+p_{000\cdot0}+p_{000\cdot1}+p_{100\cdot1}+p_{001\cdot0}+p_{001\cdot1}+p_{101\cdot1},\\ -2+p_{010\cdot0}+p_{010\cdot1}+p_{110\cdot0}+p_{110\cdot1}+p_{011\cdot0},\\ -2+p_{000\cdot0}+p_{000\cdot1}+p_{100\cdot0}+p_{100\cdot1}+p_{001\cdot0},\\ -1\end{array}\right\}$$

Upper bound =

$$\min\left\{\begin{array}{l}2-p_{000\cdot0}-p_{000\cdot1}-p_{100\cdot0}-p_{100\cdot1}-p_{101\cdot0},\\ 2-p_{000\cdot1}-p_{100\cdot0}-p_{100\cdot1}-p_{001\cdot1}-p_{101\cdot0}-p_{101\cdot1},\\ 2-p_{100\cdot0}-p_{001\cdot0}-p_{001\cdot1}-p_{101\cdot0}-p_{101\cdot1},\\ 1+p_{000\cdot0}+p_{100\cdot0}-p_{010\cdot1}-p_{110\cdot1}+p_{001\cdot0}+p_{101\cdot0}+p_{011\cdot0},\\ p_{000\cdot0}+p_{000\cdot1}+p_{100\cdot0}+p_{100\cdot1}+p_{010\cdot0}+p_{001\cdot0}+p_{001\cdot1}+p_{101\cdot0}+p_{101\cdot1}+p_{011\cdot0},\\ p_{000\cdot0}+p_{000\cdot1}+p_{100\cdot0}+p_{100\cdot1}+p_{010\cdot0}+p_{010\cdot1}+p_{110\cdot1}+p_{001\cdot0}+p_{001\cdot1}+p_{101\cdot0}+p_{101\cdot1},\\ 1\end{array}\right\}$$

Download R function for this bound (Double-click)

Back to top

## $\mathbf{NIE_{12}}$-011

Lower bound =

$$\max\left\{\begin{array}{l}-p_{000\cdot0}-p_{000\cdot1}-p_{100\cdot0}-p_{100\cdot1}-p_{001\cdot0}-p_{001\cdot1}-p_{101\cdot0}-p_{101\cdot1},\\ -2+p_{000\cdot0}+p_{000\cdot1}+p_{100\cdot0}+p_{100\cdot1}+p_{001\cdot0}+p_{001\cdot1}+p_{101\cdot0}+p_{101\cdot1}\end{array}\right\}$$

Upper bound =

$$\min\left\{\begin{array}{l}2-p_{000\cdot0}-p_{000\cdot1}-p_{100\cdot0}-p_{100\cdot1}-p_{001\cdot0}-p_{001\cdot1}-p_{101\cdot0}-p_{101\cdot1},\\ p_{000\cdot0}+p_{000\cdot1}+p_{100\cdot0}+p_{100\cdot1}+p_{001\cdot0}+p_{001\cdot1}+p_{101\cdot0}+p_{101\cdot1}\end{array}\right\}$$

Download R function for this bound (Double-click)

Back to top

## NDE-111

Lower bound =

$$\max \begin{Bmatrix} -2p_{000\cdot 1} - p_{100\cdot 1} - 2p_{010\cdot 1} - p_{110\cdot 1} - 2p_{001\cdot 1} - p_{101\cdot 1} + p_{011\cdot 0} - p_{011\cdot 1}, \\ -1 - p_{000\cdot 1} - p_{010\cdot 1} + p_{001\cdot 0} + p_{101\cdot 1} - p_{011\cdot 1}, \\ -1 - p_{000\cdot 1} + p_{010\cdot 0} + p_{110\cdot 1} - p_{001\cdot 1} - p_{011\cdot 1}, \\ -1 + p_{000\cdot 0} + p_{100\cdot 1} - p_{010\cdot 1} - p_{001\cdot 1} - p_{011\cdot 1}, \\ -p_{000\cdot 1} - p_{010\cdot 1} - p_{001\cdot 1} - p_{011\cdot 1} \end{Bmatrix}$$

Upper bound =

$$\min \begin{Bmatrix} 2 - p_{000\cdot 1} - 2p_{010\cdot 1} - p_{110\cdot 0} - p_{110\cdot 1} - p_{001\cdot 1} - p_{011\cdot 1}, \\ 2 - p_{000\cdot 1} - p_{010\cdot 1} - 2p_{001\cdot 1} - p_{101\cdot 0} - p_{101\cdot 1} - p_{011\cdot 1}, \\ p_{000\cdot 0} + p_{100\cdot 0} + p_{100\cdot 1} + p_{010\cdot 0} + p_{110\cdot 0} + p_{110\cdot 1} + p_{001\cdot 0} + p_{101\cdot 0} + p_{101\cdot 1} + p_{011\cdot 0} - p_{011\cdot 1}, \\ 1 - p_{000\cdot 1} - p_{010\cdot 1} - p_{001\cdot 1} - p_{011\cdot 1}, \\ 2 - 2p_{000\cdot 1} - p_{100\cdot 0} - p_{100\cdot 1} - p_{010\cdot 1} - p_{001\cdot 1} - p_{011\cdot 1} \end{Bmatrix}$$

Download R function for this bound (Double-click)

Back to top

## NIE$_1$-111

Lower bound =

$$\max \begin{Bmatrix} -p_{000\cdot 0} - p_{000\cdot 1} - p_{100\cdot 0} - p_{001\cdot 0} - p_{001\cdot 1} - p_{101\cdot 0}, \\ -p_{000\cdot 1} - p_{010\cdot 1} - p_{001\cdot 1} - p_{011\cdot 1}, \\ -1 + p_{000\cdot 0} + p_{100\cdot 0} - p_{010\cdot 1} + p_{001\cdot 0} + p_{101\cdot 0} - p_{011\cdot 1} \end{Bmatrix}$$

Upper bound =

$$\min \begin{Bmatrix} 2 - p_{000\cdot 0} - p_{000\cdot 1} - p_{100\cdot 0} - p_{100\cdot 1} - p_{010\cdot 1} - p_{001\cdot 0} - p_{001\cdot 1} - p_{101\cdot 0} - p_{101\cdot 1} - p_{011\cdot 1}, \\ 1 - p_{000\cdot 1} - p_{010\cdot 1} - p_{001\cdot 1} - p_{011\cdot 1}, \\ p_{000\cdot 0} + p_{100\cdot 0} + p_{100\cdot 1} + p_{001\cdot 0} + p_{101\cdot 0} + p_{101\cdot 1} \end{Bmatrix}$$

Download R function for this bound (Double-click)

Back to top

## $\text{NIE}_2$-111

Lower bound =

$$\max\left\{\begin{array}{l}-p_{000\cdot0}-p_{000\cdot1}-p_{100\cdot0}-p_{010\cdot0}-p_{010\cdot1}-p_{110\cdot0}-p_{001\cdot0}-p_{001\cdot1}-p_{101\cdot0},\\ -p_{000\cdot1}-p_{010\cdot1}-p_{001\cdot1}-p_{011\cdot1},\\ -1-p_{000\cdot1}-p_{010\cdot1}+p_{001\cdot0}+p_{101\cdot0}-p_{011\cdot1},\\ -1-p_{000\cdot1}+p_{010\cdot0}+p_{110\cdot0}-p_{001\cdot1}-p_{011\cdot1},\\ -1+p_{000\cdot0}+p_{100\cdot0}-p_{010\cdot1}-p_{001\cdot1}-p_{011\cdot1}\end{array}\right\}$$

Upper bound =

$$\min\left\{\begin{array}{l}2-p_{000\cdot0}-p_{000\cdot1}-p_{100\cdot0}-p_{100\cdot1}-p_{010\cdot1}-p_{001\cdot1}-p_{011\cdot1},\\ 1-p_{000\cdot1}-p_{010\cdot1}-p_{001\cdot1}-p_{011\cdot1},\\ 2-p_{000\cdot1}-p_{010\cdot0}-p_{010\cdot1}-p_{110\cdot0}-p_{110\cdot1}-p_{001\cdot1}-p_{011\cdot1},\\ 2-p_{000\cdot1}-p_{010\cdot1}-p_{001\cdot0}-p_{001\cdot1}-p_{101\cdot0}-p_{101\cdot1}-p_{011\cdot1},\\ p_{000\cdot0}+p_{100\cdot0}+p_{100\cdot1}+p_{010\cdot0}+p_{110\cdot0}+p_{110\cdot1}+p_{001\cdot0}+p_{101\cdot0}+p_{101\cdot1}\end{array}\right\}$$

Download R function for this bound (Double-click)

Back to top

## $\text{NIE}_{12}$-111

Lower bound =

$$\max\left\{\begin{array}{l}-p_{000\cdot0}-p_{000\cdot1}-p_{100\cdot0}-p_{001\cdot0}-p_{001\cdot1}-p_{101\cdot0},\\ -p_{000\cdot1}-p_{010\cdot1}-p_{001\cdot1}-p_{011\cdot1},\\ -1+p_{000\cdot0}+p_{100\cdot0}-p_{010\cdot1}+p_{001\cdot0}+p_{101\cdot0}-p_{011\cdot1}\end{array}\right\}$$

Upper bound =

$$\min\left\{\begin{array}{l}2-p_{000\cdot0}-p_{000\cdot1}-p_{100\cdot0}-p_{100\cdot1}-p_{010\cdot1}-p_{001\cdot0}-p_{001\cdot1}-p_{101\cdot0}-p_{101\cdot1}-p_{011\cdot1},\\ 1-p_{000\cdot1}-p_{010\cdot1}-p_{001\cdot1}-p_{011\cdot1},\\ p_{000\cdot0}+p_{100\cdot0}+p_{100\cdot1}+p_{001\cdot0}+p_{101\cdot0}+p_{101\cdot1}\end{array}\right\}$$

Download R function for this bound (Double-click)

Back to top
